# Supplementary material for: AmarDoctor: An AI-Driven, Multilingual, Voice-Interactive Digital Health Application for Primary Care Triage and Patient Management to Bridge the Digital Health Divide for Bengali Speakers
Source: arXiv:2510.24724 source file (2025-09-28)
Supplement: Supplementary file 1 [file Supplementary_Materials_1.pdf]

# Data Supplement

Supplementary Tables

**Supplementary Table 1**

Diseases presented in the vignette cases under each disease group

| Disease Group (Parent Disease) | Disease | ICD-10-CM |
|---|---|---|
| **Acne vulgaris 1.08%** | Acne vulgaris | L700 |
| **Adenomyosis 1.08%** | Adenomyosis | N80.03 |
| **Anemia 2.16%** | Anemia | D64.9 |
| | Sickle cell trait | D57. 3 |
| **Angina 1.08%** | Angina pectoris | I20 |
| **Aphthous ulcer 1.08%** | Aphthous ulcer | K12. 0 |
| **Arthritis 3.78%** | Arthritis of hip | M1315 |
| | Arthritis of knee | M1316 |
| | Chronic gouty arthritis | M1A. 9XX1 |
| | Idiopathic osteoarthritis | M19. 90 |
| | Rheumatoid arthritis | M06. 9 |
| **Asthma 1.62%** | Acute exacerbation of asthma | J45 |
| **Athlete's foot 1.08%** | Athlete's foot | B35. 3 |
| **Atrial fibrillation 1.08%** | Atrial fibrillation | I481 |
| **Bronchitis 0.54%** | Acute bronchitis | J20 |
| **Cardiac arrest 1.08%** | Cardiac arrest due to cardiac disorder | I462 |
| **Chronic obstructive pulmonary disease 0.54%** | Chronic obstructive pulmonary disease with acute lower respiratory infection | J44.0 |
| **Conjunctivitis 1.08%** | Bacterial conjunctivitis | H10 |
| **Constipation 1.08%** | Constipation | K590 |
| **Contact dermatitis 1.08%** | Contact dermatitis | L23.9 |
| **Costochondritis 1.08%** | Costochondritis | M94.0 |
| **Cystitis 0.54%** | Cystitis | N30 |
| **Dementia 1.62%** | Alzheimer's disease | G30 |
| | Presenile dementia | F03.90 |
| **Diabetes mellitus 2.16%** | Gestational diabetes mellitus | O244 |
| | Type 1 diabetes mellitus | E10 |
| **Diarrhoea 1.08%** | Diarrhoea | R19.7 |
| **Diphtheria 1.08%** | Diphtheria | A36 |
| **Diverticulitis 1.08%** | Diverticulitis of colon | K573 |
| **Diverticulosis 0.54%** | Bleeding diverticulosis | K57.31 |

**Supplementary Table 1 (Continued)**

| Disease Group (Parent Disease) | Disease | ICD-10-CM |
|---|---|---|
| **Ear infection 1.08%** | Otitis media | H66.9 |
| **Eczema 1.08%** | Eczema | L20 |
| **Embolism 1.08%** | Pulmonary embolism | I26 |
| **Endometriosis 1.08%** | Endometriosis | N80 |
| **Epididymitis 1.08%** | Epididymitis | N451 |
| **Epilepsy 1.08%** | Epilepsy | G40 |
| **Epistaxis 0.54%** | Epistaxis | R040 |
| **Fibromyalgia 1.08%** | Fibromyalgia | M797 |
| **Flu 1.08%** | Common flu | M94.0 |
| **Fungal infection 1.08%** | Oral thrush | B379 |
| | Vaginal thrush | B37.3 |
| **Gallstone 1.08%** | Acute cholecystitis | K810 |
| **Gastritis 2.16%** | Acute gastritis | K290 |
| | Stomach ulcer | K25.9 |
| **Gout 1.08%** | Gout | M10 |
| **Headache 0.54%** | Tension-type headache | G442 |
| **Heart disease 2.70%** | Cardiomyopathy | I42 |
| | Coronary artery spasm | I2541 |
| | Hypertensive heart disease | I11 |
| **Heart failure 2.70%** | Systolic heart failure | I5020 |
| | Chronic diastolic heart failure | I5032 |
| | Congestive heart failure | I50 |
| | Hypertensive heart failure | I508 |
| **Hepatitis 2.16%** | Acute hepatitis C | B171 |
| | Acute type B viral Hepatitis | B16.9 |
| **Hyperemesis gravidarum 1.08%** | Hyperemesis gravidarum | O2689 |
| **Hyperthyroidism 1.08%** | Hyperthyroidism | E05 |
| **Hypothyroidism 1.08%** | Hypothyroidism | E03.9 |
| **Hypoglycemia 1.08%** | Hypoglycemia | E08.641 |
| **Inflammatory bowel disease 2.16%** | Crohn's disease | K5000 |
| | Ulcerative colitis | K51 |
| **Irritable bowel syndrome 1.08%** | Irritable bowel syndrome | K58 |
| **Kidney disease 2.70%** | Acute renal failure due to acute cortical necrosis | N17 |
| | Chronic kidney disease | N18 |
| | Polycystic kidney disease | Q61.2 |
| **Kidney stone 1.08%** | Kidney stone | N20.0 |
| **Laryngitis 1.08%** | Laryngitis | J04.0 |

**Supplementary Table 1 (Continued)**

| Disease Group (Parent Disease) | Disease | ICD-10-CM |
|---|---|---|
| **Liver disease 2.16%** | Cirrhosis of liver | K74.5 |
| | Non-alcoholic fatty liver disease | K75.8 |
| **Lung disease 1.08%** | Pulmonary hypertension | I27.0 |
| **Mastitis 1.08%** | Mastitis | N610 |
| **Meningitis 1.08%** | Meningitis | G02 |
| **Migraine 1.08%** | Migraine | G43 |
| **Mosquito borne disease 2.16%** | Chikungunya fever | A920 |
| | Falciparum malaria | B50.9 |
| **Osteoporosis 1.08%** | Osteoporosis | M81.0 |
| **Ovarian cyst 1.08%** | Ovarian cyst | Q501 |
| **Pelvic inflammatory disease 0.54%** | Vaginitis | N760 |
| **Piles 1.08%** | Piles | K64 |
| **Pre-eclampsia 1.08%** | Pre-eclampsia | O14 |
| **Prolapse 1.08%** | Uterovaginal prolapse | N81.3 |
| **Psoriasis 1.08%** | Psoriasis | L40 |
| **Radiculopathy 1.08%** | Cervical Radiculopathy | M5412 |
| **Renal disorder 0.54%** | Renal disorder due to type 2 diabetes | E1122 |
| **Respiratory infection 2.70%** | Acute lower respiratory tract infection | J22 |
| | Acute upper respiratory infection | J06.9 |
| **Retinopathy 0.54%** | Diabetic retinopathy associated with type 1 diabetes mellitus | E10355 |
| **Rhabdomyolysis 0.54%** | Rhabdomyolysis | M6282 |
| **Scabies 1.08%** | Scabies | B86 |
| **Sciatica 2.16%** | Low back pain | M545 |
| | Sciatica | M543 |
| **Sinusitis 1.08%** | Acute sinusitis | J01 |
| **Sleep apnea 1.08%** | Sleep apnea | G473 |
| **Spondylosis 1.08%** | Spondylosis | M47 |
| **Stroke 3.78%** | Aphasia | R4701 |
| | Hemorrhagic stroke | I60 |
| | Ischemic stroke | I609 |
| | Transient ischemic stroke | G45.9 |
| **Stye 1.08%** | Stye | H00.025 |
| **Thread worms 1.08%** | Thread worms | B80 |
| **Tuberculosis 1.08%** | Pulmonary tuberculosis | A150 |
| **Typhoid 1.08%** | Typhoid and paratyphoid fevers | A01 |
| **Urinary tract infectious disease 1.08%** | Urinary tract infection | N390 |

**Supplementary Table 2**

Diseases Covered by AmarDoctor with ICD-10-CM Codes

| **Disease Name** | **Disease Group** | **ICD-10-CM** |
|---|---|---|
| Acne vulgaris | Acne vulgaris | L700 |
| Acute bronchitis | Bronchitis | J20 |
| Acute cholecystitis | Gallstone | K810 |
| Acute diastolic heart failure | Heart failure | I5031 |
| Acute exacerbation of asthma | Asthma | J45 |
| Acute gastritis | Gastritis | K290 |
| Acute hemorrhagic gastritis | Gastritis | K29 |
| Acute hepatitis A | Hepatitis | B15 |
| Acute hepatitis B | Hepatitis | B16 |
| Acute hepatitis C | Hepatitis | B171 |
| Acute hepatitis E | Hepatitis | B172 |
| Acute lower respiratory tract infection | Respiratory infection | J22 |
| Acute mycoplasmal bronchitis | Bronchitis | J218 |
| Acute parainfluenza virus bronchitis | Bronchitis | J210 |
| Acute renal failure due to acute cortical necrosis | Renal failure | N17 |
| Acute renal failure syndrome | Kidney disease | N17.9 |
| Acute renal papillary necrosis with renal failure | Renal failure | N17.0 |
| Acute sinusitis | Sinusitis | J01 |
| Acute systolic heart failure | Heart failure | I5021 |
| Acute tonsillitis | Tonsillitis | J03 |
| Acute type B viral hepatitis | Hepatitis | B16.9 |
| Acute upper respiratory infection | Respiratory infection | J06.9 |
| Acute upper respiratory infection of multiple sites | Respiratory infection | J06.8 |
| Adenomyosis | Adenomyosis | N80.03 |
| Alcoholic gastritis | Gastritis | K292 |
| Alcoholic hepatitis | Hepatitis | K701 |
| Allergic arthritis | Arthritis | M13.869 |
| Alzheimer's disease | Dementia | G30 |
| Amyotrophy due to type 2 diabetes mellitus | Amyotrophy due to type 2 diabetes mellitus | E1144 |
| Anemia | Anemia | D64.9 |
| Angina decubitus | Angina | I20.9 |
| Angina pectoris | Angina | I20 |
| Aphasia | Stroke | R4701 |
| Aphthous ulcer | Aphthous ulcer | K12.0 |
| Arthritis | Arthritis | R06.81 |
| Arthritis of elbow | Arthritis | M1312 |

**Supplementary Table 2 (Continued)**

| **Disease Name** | **Disease Group** | **ICD-10-CM** |
|---|---|---|
| Arthritis of hand | Arthritis | M1314 |
| Arthritis of hip | Arthritis | M1315 |
| Arthritis of knee | Arthritis | M1316 |
| Arthritis of wrist | Arthritis | M1313 |
| Asthma | Asthma | J45 |
| Athlete's foot | Athlete's foot | B35.3 |
| Atrial fibrillation | Atrial fibrillation | I481 |
| Atrial fibrillation and flutter | Atrial fibrillation | I48 |
| Atrophic gastritis | Gastritis | K29.4 |
| Bacterial arthritis | Arthritis | M00 |
| Bacterial conjunctivitis | Conjunctivitis | H10 |
| Bacterial meningitis | Meningitis | G00.9 |
| Benign hypertensive heart disease with congestive cardiac failure | Heart failure | I110 |
| Benign hypertensive heart disease with congestive heart failure | Heart failure | I110 |
| Biventricular heart failure | Heart failure | I5082 |
| Bleeding diverticulosis | Diverticulosis | K57.31 |
| Bronchitis | Bronchitis | J20.9 |
| Cardiac arrest | Cardiac arrest | I46 |
| Cardiac arrest as a complication of care | Cardiac arrest | I468 |
| Cardiac arrest due to cardiac disorder | Cardiac arrest | I462 |
| Cardiomyopathy | Heart disease | I42 |
| Central sleep apnea syndrome | Sleep apnea | G47.31 |
| Cervical disc disorder with radiculopathy | Radiculopathy | M501 |
| Cervical radiculopathy | Radiculopathy | M5412 |
| Cervical spondylosis | Spondylosis | M4303 |
| Cervical spondylosis with myelopathy | Spondylosis | M47812 |
| Cervical spondylosis with radiculopathy | Radiculopathy | M47812 |
| Cervicitis | Pelvic inflammatory disease | N72 |
| Chikungunya fever | Mosquito borne disease | A920 |
| Cholecystitis | Gallstone | K81 |
| Chronic asthmatic bronchitis | Bronchitis | J44 |
| Chronic atrial fibrillation | Atrial fibrillation | I482 |
| Chronic bronchitis | Bronchitis | J41.0 |
| Chronic cholecystitis | Gallstone | K811 |
| Chronic diastolic heart failure | Heart failure | I5032 |
| Chronic frontal sinusitis | Sinusitis | J321 |

**Supplementary Table 2 (Continued)**

| Disease Name | Disease Group | ICD-10-CM |
|---|---|---|
| Chronic gastritis | Gastritis | K29.5 |
| Chronic gouty arthritis | Arthritis | M1A.9XX1 |
| Chronic hepatitis | Hepatitis | K73.9 |
| Chronic idiopathic pulmonary fibrosis | Chronic obstructive pulmonary disease | J84.112 |
| Chronic ischemic heart disease | Heart disease | I25 |
| Chronic kidney disease | Kidney disease | N18 |
| Chronic kidney disease due to hypertension | Kidney disease | I12.9 |
| Chronic kidney disease due to type 2 diabetes mellitus | Kidney disease | E11.22 |
| Chronic kidney disease stage 2 | Kidney disease | N182 |
| Chronic kidney disease stage 3 | Kidney disease | N1830 |
| Chronic kidney disease stage 4 | Kidney disease | N184 |
| Chronic kidney disease stage 5 | Kidney disease | N185 |
| Chronic kidney disease stage 5 due to hypertension | Kidney disease | I12.0 |
| Chronic maxillary sinusitis | Sinusitis | J320 |
| Chronic obstructive lung disease | Chronic obstructive pulmonary disease | J44.9 |
| Chronic obstructive pulmonary disease with acute lower respiratory infection | Chronic obstructive pulmonary disease | J44.0 |
| Chronic pulmonary edema | Chronic obstructive pulmonary disease | J811 |
| Chronic pulmonary heart disease | Heart disease | I27.9 |
| Chronic sinusitis | Sinusitis | J32 |
| Chronic superficial gastritis | Gastritis | K293 |
| Chronic uterine inflammatory disease | Pelvic inflammatory disease | N71.1 |
| Cirrhosis of liver | Liver disease | K74.5 |
| Climacteric arthritis | Arthritis | M13.849 |
| Common cold | Flu | M94.0 |
| Congenital anomaly of coronary artery | Heart disease | Q24.5 |
| Congenital renal failure | Kidney disease | P960 |
| Congestive heart failure | Heart failure | I50 |
| Congestive rheumatic heart failure | Heart failure | I0981 |
| Constipation | Constipation | K590 |
| Contact dermatitis | Contact dermatitis | L23.9 |
| Coronary arteriosclerosis in native artery | Heart disease | I25.119 |
| Coronary artery spasm | Heart disease | I2541 |

**Supplementary Table 2 (Continued)**

| **Disease Name** | **Disease Group** | **ICD-10-CM** |
|---|---|---|
| Costochondritis | Costochondritis | M94. 0 |
| Cough variant asthma | Asthma | J45991 |
| Crohn's disease | Inflammatory bowel disease | K5000 |
| Cystitis | Cystitis | N30 |
| Dementia | Dementia | F03. 90 |
| Dengue | Mosquito borne disease | A90 |
| Diabetic dermopathy associated with diabetes mellitus type 2 | Diabetes dermopathy | E11. 62 |
| Diabetic oculopathy associated with type 1 diabetes mellitus | Diabetic oculopathy | E10.3 |
| Diabetic oculopathy associated with type 2 diabetes mellitus | Diabetic oculopathy | E11.3 |
| Diabetic retinopathy associated with type 1 diabetes mellitus | Retinopathy | E10355 |
| Diarrhoea | Diarrhoea | R19. 7 |
| Diastolic heart failure | Heart failure | I503 |
| Dilated cardiomyopathy | Heart disease | I420 |
| Diphtheria | Diphtheria | A36 |
| Dissection of coronary artery | Heart disease | I2542 |
| Diverticulitis of colon | Diverticulitis | K573 |
| Eczema | Eczema | L20 |
| Endometriosis | Endometriosis | N80 |
| Enteropathic arthritis | Inflammatory bowel disease | M07.60 |
| Enterovirus meningitis | Meningitis | A87.0 |
| Eosinophilic asthma | Asthma | J8283 |
| Epididymitis | Epididymitis | N451 |
| Epilepsy | Epilepsy | G40 |
| Epistaxis | Epistaxis | R040 |
| Exacerbation of intermittent asthma | Asthma | J45.21 |
| Exercise-induced asthma | Asthma | J45.990 |
| Falciparum malaria | Mosquito borne disease | B50.9 |
| Fibromyalgia | Fibromyalgia | M797 |
| Fistula of intestine due to ulcerative colitis | Inflammatory bowel disease | K51.913 |
| Foot ulcer due to type 2 diabetes mellitus | Foot ulcer | E11.621 |
| Frontotemporal dementia | Dementia | G310 |
| Gastritis | Gastritis | K29.70 |
| Generalized convulsive epilepsy | Epilepsy | G40.309 |
| Generalized epilepsy | Epilepsy | G40.309 |
| Genitourinary tract infection in pregnancy | Urinary tract infection | O23.40 |

**Supplementary Table 2 (Continued)**

| **Disease Name** | **Disease Group** | **ICD-10-CM** |
|---|---|---|
| Gestational diabetes mellitus | Diabetes mellitus | O244 |
| Gout | Gout | M10 |
| Hay fever | Allergy | J30.1 |
| Heart attack | Myocardial infarction | I21.9 |
| Heart failure | Heart failure | I50 |
| Heat stroke and sunstroke | Stroke | T67.01 |
| Hemiplegic migraine | Migraine | G434 |
| Hemorrhagic stroke | Stroke | I60 |
| Hyperemesis gravidarum | Hyperemesis gravidarum | O2689 |
| Hyperglycemia due to type 1 diabetes mellitus | Hyperglycemia | E10.65 |
| Hyperglycemia due to type 2 diabetes mellitus | Hyperglycemia | E11.65 |
| Hypertension | Hypertension | I10 |
| Hypertensive heart and renal disease with (congestive) heart failure | Heart failure | I1310 |
| Hypertensive heart and renal disease with both (congestive) heart failure and renal failure | Heart failure | I1311 |
| Hypertensive heart disease | Heart disease | I11 |
| Hypertensive heart disease with congestive heart failure | Heart failure | I110 |
| Hypertensive heart failure | Heart failure | I508 |
| Hyperthyroidism | Hyperthyroidism | E05 |
| Hypertrophic cardiomyopathy | Heart disease | I42.1 |
| Hypertrophic gastritis | Gastritis | K29 |
| Hypertrophic obstructive cardiomyopathy | Heart disease | I421 |
| Hypoglycemia | Hypoglycemia | E08.641 |
| Hypoglycemia due to type 1 diabetes mellitus | Hypoglycemia | E1064 |
| Hypoglycemia due to type 2 diabetes mellitus | Hypoglycemia | E1164 |
| Hypoglycemic coma in type 1 diabetes mellitus | Hyperglycemia coma | E10641 |
| Hypothyroidism | Hypothyroidism | E03.9 |
| Hypothyroidism caused by drug | Hypothyroidism | E03.2 |
| Iatrogenic hypothyroidism | Hypothyroidism | E03.2 |
| Idiopathic osteoarthritis | Arthritis | M19.90 |
| Influenza | Flu | J09 |
| Iodine hypothyroidism | Hypothyroidism | E01.8 |
| Iron deficiency anemia | Anemia | D50 |
| Irritable bowel syndrome | Irritable bowel syndrome | K58 |
| Ischemic stroke | Stroke | I609 |
| Juvenile rheumatoid arthritis | Arthritis | M080 |
| Ketoacidosis in type 1 diabetes mellitus | Ketoacidosis | E101 |

**Supplementary Table 2 (Continued)**

| **Disease Name** | **Disease Group** | **ICD-10-CM** |
|---|---|---|
| Ketoacidosis in type 2 diabetes mellitus | Ketoacidosis | E111 |
| Kidney stone | Kidney stone | N20.0 |
| Laryngitis | Laryngitis | J04.0 |
| Left heart failure | Heart failure | I501 |
| Left sided ulcerative colitis | Inflammatory bowel disease | K51.5 |
| Low back pain | Sciatica | M545 |
| Lumbar spondylosis | Spondylosis | M47.816 |
| Lumbar spondylosis with myelopathy | Spondylosis | M47.16 |
| Mastitis | Mastitis | N610 |
| Meningitis | Meningitis | G02 |
| Menstrual migraine | Migraine | G438 |
| Migraine | Migraine | G43 |
| Migraine with aura | Migraine | G431 |
| Migraine without aura | Migraine | G430 |
| Neurologic disorder associated with type 2 diabetes mellitus | Neurologic disorder | E11.4 |
| Neurological disorder associated with type 1 diabetes mellitus | Neurological disorder | E10.49 |
| Non-alcoholic fatty liver disease | Liver disease | K75.8 |
| Obstructive sleep apnea syndrome | Sleep apnea | G47.39 |
| Ophthalmoplegic migraine | Migraine | G43B |
| Oral thrush | Fungal infection | B379 |
| Osteoarthritis | Arthritis | M19.9 |
| Osteoarthritis of elbow | Arthritis | M19.02 |
| Osteoarthritis of hip | Osteoarthritis | M16 |
| Osteoarthritis of knee | Arthritis | M17 |
| Osteoarthritis of wrist | Arthritis | M19.03 |
| Osteoporosis | Osteoporosis | M81.0 |
| Otitis media | Ear infection | H66.9 |
| Ovarian cyst | Ovarian cyst | Q501 |
| Paroxysmal atrial fibrillation | Atrial fibrillation | I480 |
| Pelvic inflammatory disease | Pelvic inflammatory disease | N73.9 |
| Persistent atrial fibrillation | Atrial fibrillation | I481 |
| Pharyngitis | Pharyngitis | J02.9 |
| Piles | Piles | K64 |
| Pneumococcal meningitis | Meningitis | G001 |

**Supplementary Table 2 (Continued)**

| **Disease Name** | **Disease Group** | **ICD-10-CM** |
|---|---|---|
| Polycystic kidney disease | Kidney disease | Q61.2 |
| Polyneuropathy due to type 1 diabetes mellitus | Polyneuropathy | E1042 |
| Polyneuropathy due to type 2 diabetes mellitus | Polyneuropathy | Z79.4 |
| Post traumatic osteoarthritis | Arthritis | M19.92 |
| Postablative hypothyroidism | Hypothyroidism | E89.0 |
| Postpartum acute renal failure | Kidney disease | O90.4 |
| Postpartum cardiomyopathy | Heart disease | O90.3 |
| Pre-eclampsia | Pre-eclampsia | O14 |
| Presenile dementia | Dementia | F03.90 |
| Primary central sleep apnea | Sleep apnea | G4731 |
| Primary gout | Gout | M10.9 |
| Psoriasis | Psoriasis | L40 |
| Pulmonary arterial hypertension | Lung disease | I27.21 |
| Pulmonary embolism | Embolism | I26 |
| Pulmonary hypertension | Lung disease | I27.0 |
| Pulmonary tuberculosis | Tuberculosis | A150 |
| Quartan malaria | Mosquito borne disease | B52 |
| Rectal hemorrhage due to ulcerative colitis | Inflammatory bowel disease | K51.911 |
| Refractory epilepsy | Epilepsy | G40.919 |
| Renal disorder associated with type 1 diabetes mellitus | Kidney disease | E1022 |
| Renal disorder due to type 2 diabetes mellitus | Renal disorder | E1122 |
| Renal failure syndrome | Renal failure | N17.9 |
| Restrictive cardiomyopathy | Heart disease | I42.5 |
| Rhabdomyolysis | Rhabdomyolysis | M6282 |
| Rheumatoid arthritis | Arthritis | M06. 9 |
| Rheumatoid arthritis - hand joint | Arthritis | M0844 |
| Rheumatoid arthritis of hip | Arthritis | M0845 |
| Rheumatoid arthritis of knee | Arthritis | M0846 |
| Right heart failure, unspecified | Heart failure | I50810 |
| SARS COVID-19 | Viral infection | U071 |
| Scabies | Scabies | B86 |
| Sciatica | Sciatica | M543 |
| Secondary gout | Gout | M104 |
| Secondary pulmonary arterial hypertension | Lung disease | I2721 |
| Secondary pulmonary hypertension | Lung disease | I27.21 |

**Supplementary Table 2 (Continued)**

| **Disease Name** | **Disease Group** | **ICD-10-CM** |
|---|---|---|
| Sickle cell trait | Anemia | D57.3 |
| Sleep apnea | Sleep apnea | G473 |
| Sore throat | Flu | R07.0 |
| Spondylosis | Spondylosis | M47 |
| Stomach ulcer | Gastritis | K25.9 |
| Stye | Stye | H00.025 |
| Systolic heart failure | Heart failure | I5020 |
| Takotsubo cardiomyopathy | Heart disease | I51.81 |
| Tension-type headache | Headache | G442 |
| Thread worms | Thread worms | B80 |
| Transient ischemic attack | Stroke | G45.9 |
| Tuberculous arthritis | Arthritis | A18.02 |
| Type 1 diabetes mellitus | Diabetes mellitus | E10 |
| Type 1 diabetes mellitus uncontrolled | Diabetes mellitus | E10.65 |
| Type 1 diabetes mellitus with ulcer | Foot ulcer | E10621 |
| Type 2 diabetes mellitus | Diabetes mellitus | E11 |
| Type 2 diabetes mellitus uncontrolled | Diabetes mellitus | E11.65 |
| Type 2 diabetes mellitus with arthropathy | Type 2 diabetes mellitus with arthropathy | E11618 |
| Type 2 diabetes mellitus with gangrene | Foot ulcer | E1152 |
| Type 2 diabetes mellitus with neuropathic arthropathy | Neuropathic arthropathy | E11610 |
| Type 2 diabetes mellitus with peripheral angiopathy | Peripheral angiopathy | E1151 |
| Type 2 diabetes mellitus with ulcer | Foot ulcer | E11621 |
| Typhoid | Typhoid | A010 |
| Typhoid and paratyphoid fevers | Typhoid | A01 |
| Ulcerative colitis | Inflammatory bowel disease | K51 |
| Urinary tract infection following delivery | Urinary tract infection | O862 |
| Urinary tract infection in pregnancy | Urinary tract infection | O23.40 |
| Urinary tract infectious disease | Urinary tract infection | N390 |
| Uterovaginal prolapse | Prolapse | N81.3 |
| Vaginal thrush | Fungal infection | B37.3 |
| Vaginitis | Pelvic inflammatory disease | N760 |
| Vascular dementia | Dementia | F01 |
| Viral conjunctivitis | Conjunctivitis | B30 |
| Viral hepatitis | Hepatitis | B19 |
| Viral meningitis | Meningitis | A87 |

**Supplementary Table 3 (Overview of vignette cases: age and gender distribution, and representation of different medical specialization)**

| **Age** | 18 years to 78 years |
|---|---|
| **Male/Female** | 51%/49% |
| **Specialization Classification** | |
| Medicine / General Physician | 18.37% |
| Neuromedicine | 11.89% |
| Cardiology | 8.65% |
| Gastroenterology | 7.02% |
| Rheumatology | 7.02% |
| Respiratory / Chest Disease | 6.49% |
| Gynaecology | 5.95% |
| Diabetes / Endocrinology | 5.95% |
| Skin / Dermatology | 5.40% |
| ENT | 4.86% |
| Hepatology | 4.32% |
| Nephrology | 3.24% |
| Neuromedicine / Orthopedic | 2.16% |
| Urology | 2.16% |
| Haematology | 2.16% |
| EYE / Ophthalmology | 2.16% |
| General Surgery | 1.08% |
| Gynaecology / Obstetric | 1.08% |

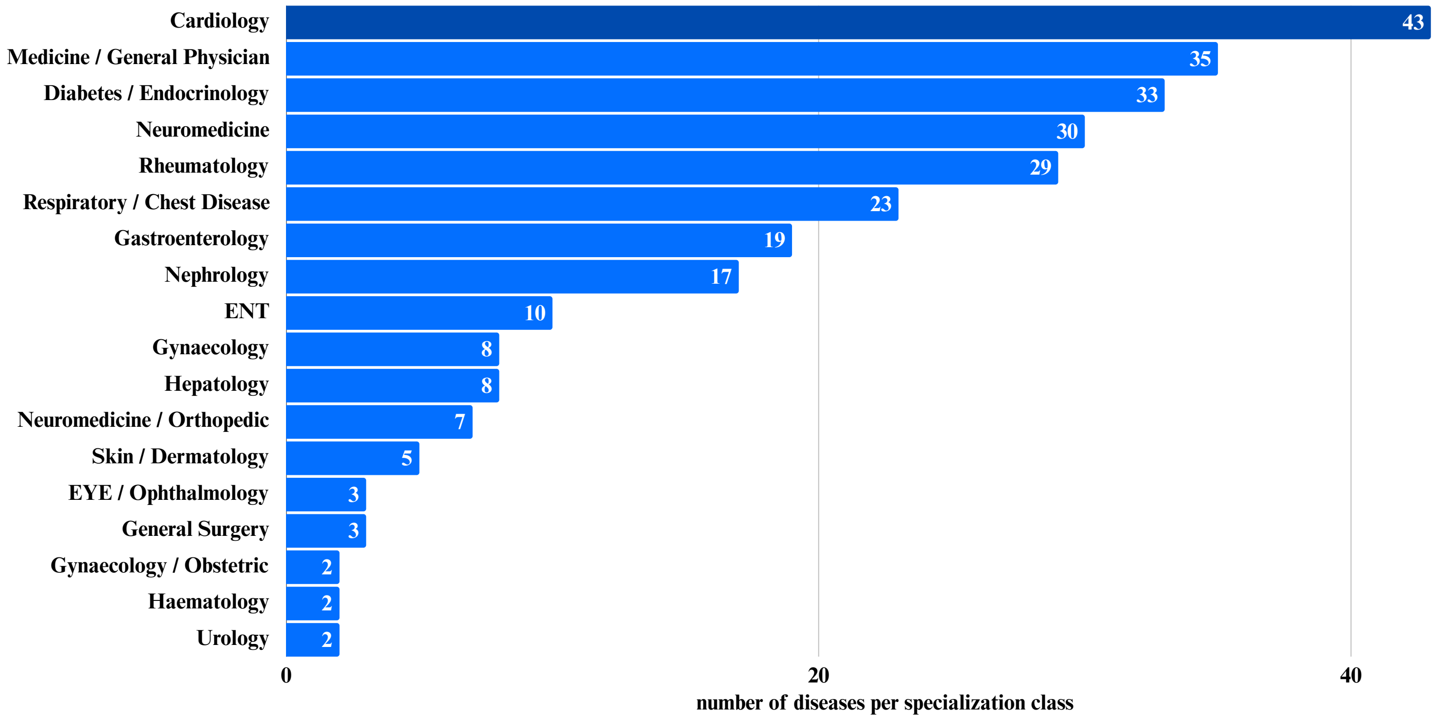


Figure 1: Overall distribution of diseases under each specialization class
