# Supplementary material for: AmarDoctor: An AI-Driven, Multilingual, Voice-Interactive Digital Health Application for Primary Care Triage and Patient Management to Bridge the Digital Health Divide for Bengali Speakers
Source: arXiv:2510.24724 source file (2025-09-28)
Supplement: Supplementary file 2 [file Supplementary_Materials_2.pdf]

Supplementary Table 4

# Patient Vignette

| Patient ID | Gold Standard<br>Main Diagnosis | Gold Standard<br>Main Specialization | Sex | Age | Family<br>History | Medical<br>History | Any Current Medicatior | Allergies | Any Other Remarks | Chief Complaints | Additional_Symptoms |
|---|---|---|---|---|---|---|---|---|---|---|---|
| Patient 2 | Bronchitis | Respiratory / Chest Disease | Male | 42 | asthma | | | | | cough with phlegm for 1-3 weeks<br>green or yellow cough<br>mild fever | nasal congestion \| YES<br>headache \| YES<br>muscle pain \| NO<br>body ache \| NO<br>tiredness or fatigue \| YES<br>sleepiness \| YES<br>poor appetite \| YES<br>diarrhoea \| NO<br>nausea and vomiting \| NO<br>pain in abdomen \| NO<br>chills or shiver \| YES<br>high fever \| NO<br>shortness of breath \| YES<br>wheezing \| YES<br>nasal congestion \| NO |
| Patient 6 | Gallstone | General Surgery | Female | 28 | heart_disease | | | | | pain in upper abdomen<br>vomiting<br>nausea and vomiting | swelling in your legs ankles or feet \| NO<br>belching \| NO<br>urine retention \| NO<br>feeling of fullness in abdomen \| NO<br>pain in upper-right abdomen that radiates to<br>back and shoulder \| YES<br>high fever \| NO<br>tenderness in abdomen \| YES<br>sweating \| YES<br>yellow skin and eyes \| NO<br>poor appetite \| YES<br>chills or shiver \| YES<br>bulge in the tummy \| YES<br>diarrhoea \| NO<br>cramping in abdomen from gallstones \| YES<br>constipation \| NO |
| Patient 7 | Gallstone | General Surgery | Female | 33 | | diabetes | Oral hypoglycaemic agents | | | nausea and vomiting<br>pain in upper-right abdomen<br>fever | dull pain in upper-right abdomen \| YES<br>high fever \| YES<br>tenderness in abdomen \| YES<br>sweating \| YES<br>yellow skin and eyes \| NO<br>poor appetite \| NO<br>chills or shiver \| NO<br>bulge in the tummy \| YES<br>restricted movement \| NO<br>diarrhoea \| NO<br>cramping in abdomen from gallstones \| YES<br>constipation \| YES<br>discomfort in abdomen \| YES<br>recurrent infections \| YES<br>sharp pains or cramps in abdomen \| YES |
| Patient 11 | Asthma | Respiratory / Chest Disease | Male | 23 | | asthma | | Tobacco | | wheezing<br>persistent cough<br>rapid breathing | coughing up blood \| NO<br>shortness of breath \| YES<br>cough with phlegm \| YES<br>recurring chest infection \| YES<br>chest pain \| YES<br>blue or gray skin color due to low oxygen levels \| YES<br>weight loss \| NO<br>acute episodes \| YES<br>lethargy \| YES<br>chills or shiver \| NO<br>fever \| YES<br>chest pressure \| YES<br>respiratory distress \| YES<br>difficulty breathing \| YES<br>tiredness or fatigue \| YES |
| Patient 12 | Asthma | Respiratory / Chest Disease | Female | 30 | asthma | | | Dust, pets | History of exposure<br>to allergens | wheezing<br>dry cough<br>mild fever | shortness of breath at rest \| YES<br>persistent cough \| YES<br>blue or gray skin color due to low oxygen levels \| YES<br>acute episodes \| YES<br>lethargy \| YES |

# Supplementary Table 4

| | | | | | | | | | | | |
|---|---|---|---|---|---|---|---|---|---|---|---|
| Patient 16 | Gastritis | Gastroenterology | Male | 25 | | | | | History of taking oily and spicy food | vomiting<br>nausea and vomiting<br>burning in your abdomen | swelling in your legs ankles or feet \| NO<br>urine retention \| NO<br>pain in abdomen \| YES<br>dark stool from digested blood \| NO<br>pain in upper abdomen \| YES<br>belching \| NO<br>indigestion \| YES<br>diarrhoea \| NO<br>chills or shiver \| NO<br>discomfort in upper abdomen \| YES<br>dull pain in upper abdomen \| YES<br>feeling of fullness or burning in your abdomen \| YES<br>bloating \| YES<br>weight loss \| YES<br>tenderness in abdomen \| NO |
| Patient 17 | Gastritis | Gastroenterology | Male | 56 | heart_disease | | | | | vomiting<br>feeling of fullness or burning in your abdomen<br>nausea and vomiting | swelling in your legs ankles or feet \| NO<br>high blood pressure \| NO<br>pain in abdomen \| NO<br>urine retention \| NO<br>pelvic pain \| NO<br>belching \| NO<br>poor appetite \| YES<br>bloating \| YES<br>diarrhoea \| NO<br>chills or shiver \| YES<br>vomiting blood \| NO<br>tenderness in the affected area \| NO<br>discomfort \| YES<br>constipation \| NO<br>cramping \| NO |
| Patient 26 | Hepatitis | Hepatology | Male | 33 | | | | | History of blood transfusion after an accident 1 year back | yellow skin and eyes<br>light clay-colored stool<br>dull pain in abdomen | diarrhoea \| NO<br>joint pain \| YES<br>vomiting \| YES<br>live or travelled recently to areas prone to viral fevers like dengue malaria chikungunya or high prevalence of hepatitis (e.g. India or Africa) \| YES<br>belching \| NO<br>feeling of fullness or burning in your abdomen \| NO<br>fluid in the abdomen \| YES<br>poor appetite \| YES<br>chills or shiver \| NO<br>vomiting blood \| NO<br>tenderness in the affected area \| NO<br>discomfort in abdomen \| YES<br>constipation \| YES<br>unexplained fatigue \| YES |
| Patient 27 | Hepatitis | Hepatology | Male | 45 | diabetes | | | | | light clay-colored stool<br>itching<br>yellow skin and eyes | lice on head \| NO<br>malaise \| YES<br>live or travelled recently to areas prone to viral fevers like dengue malaria chikungunya or high prevalence of hepatitis (e.g. India or Africa) \| YES<br>mild fever \| YES<br>pain in upper abdomen \| YES<br>diarrhoea \| NO<br>constipation \| NO<br>nausea and vomiting \| NO<br>cloudy or bloody urine \| YES<br>headache \| YES<br>muscle pain \| NO<br>poor appetite \| YES<br>tiredness or fatigue \| YES<br>itchy skin \| YES<br>easy bruising \| NO |
| Patient 36 | Respiratory infectic | Respiratory / Chest Disease | Male | 33 | | | | | | severe cough<br>wheezing<br>fever | cough with phlegm \| YES<br>chills or shiver \| YES<br>shortness of breath at rest \| YES<br>sore throat \| NO<br>nasal congestion \| YES<br>chest pressure \| YES<br>tiredness or fatigue \| YES<br>lethargy \| YES<br>runny nose \| NO<br>malaise \| YES<br>persistent cough \| YES<br>chest discomfort \| YES<br>chest pain worsened by breathing \| YES<br>rib pain \| YES<br>throbbing headache \| NO |

# Supplementary Table 4

| | | | | | | | | | | | |
|---|---|---|---|---|---|---|---|---|---|---|---|
| Patient 37 | Respiratory infectic | Respiratory / Chest Disease | Female | 23 | COPD | | | | | wheezing<br>cough with phlegm<br>shortness of breath | shortness of breath at rest \| NO<br>chills or shiver \| NO<br>chest tightness \| YES<br>pale or bluish skin \| YES<br>chest pain worsened by breathing \| NO<br>nasal congestion \| YES<br>anxiety \| YES<br>depression \| YES<br>sore throat \| NO<br>headache \| YES<br>rapid heartbeat \| YES<br>chest discomfort \| YES |
| Patient 51 | Kidney disease | Nephrology | Female | 33 | diabetes | | | | History of abruptio<br>placenta | swelling in your legs ankles or feet<br>shortness of breath<br>decreased urine output | urine retention \| YES<br>tiredness or fatigue \| YES<br>nausea and vomiting \| YES<br>back pain \| YES<br>confusion \| NO |
| Patient 52 | Kidney disease | Nephrology | Male | 45 | | diabetes | Insulin | | | urine retention<br>shortness of breath<br>swelling in your legs ankles or feet | high blood pressure \| YES<br>confusion \| YES |
| Patient 71 | Sinusitis | ENT | Male | 27 | | | | | | throbbing headache<br>thick discolored discharge from nose<br>runny or stuffy nose | bleeding from your nose without any injury \| NO<br>sinus pain \| YES<br>sudden severe headache \| YES<br>fever \| NO<br>live or travelled recently to areas prone to diseases<br>like meningitis (e.g. sub-Saharan Africa) \| NO<br>pale or mottled skin \| NO<br>cold hands and feet \| NO<br>pain between eyes and on the side of the nose relieved<br>by nasal decongestant \| YES<br>stiffness or pain in the neck \| NO<br>nasal inflammation \| YES<br>drowsiness \| YES<br>sensitivity to light \| YES<br>malaise \| YES<br>arm pain or discomfort \| YES<br>cough with phlegm \| NO |
| Patient 72 | Sinusitis | ENT | Female | 45 | hypertension | | | | | runny or stuffy nose<br>headache<br>thick discolored discharge from nose | cough with phlegm \| NO<br>dry cough \| NO<br>chills or shiver \| NO<br>bleeding from your nose without any injury \| NO<br>sore throat \| NO<br>muscle pain \| NO<br>tiredness or fatigue \| NO<br>body ache \| YES<br>sinus pain \| YES<br>irritability \| YES<br>pain between eyes and on the side of the nose relieved<br>by nasal decongestant \| NO<br>dehydration \| YES<br>arm pain or discomfort \| YES<br>cough with phlegm \| NO |
| Patient 77 | Anemia | Haematology \|<br>Medicine / General Physician | Female | 25 | | | | | History of 4 children | pale skin<br>lethargy or extreme fatigue<br>weakness | fainting \| YES<br>shakiness \| NO<br>lightheadedness \| YES<br>dark stool from digested blood \| YES<br>irregular heartbeat \| YES<br>seizures \| NO<br>tingling in fingers or hands \| YES<br>confusion \| NO<br>low blood pressure \| NO<br>cold hands and feet \| YES<br>arm pain or discomfort \| YES<br>cough with phlegm \| NO |
| Patient 78 | Anemia | Haematology \|<br>Medicine / General Physician | Female | 35 | hypertension | | | | | unexplained fatigue<br>dizziness<br>weakness | lethargy or extreme fatigue \| YES<br>iron deficiency \| YES<br>pale skin \| YES<br>lightheadedness \| YES<br>dark stool from digested blood \| NO<br>shortness of breath \| YES<br>inflammation or soreness of your tongue \| YES<br>rapid heartbeat \| YES<br>cold hands and feet \| YES<br>bleeding easily \| NO<br>brittle nails \| YES<br>malnutrition \| YES<br>nausea and vomiting \| YES<br>depression \| YES<br>sadness \| YES |

Supplementary Table 4

| | | | | | | | | | | | |
|---|---|---|---|---|---|---|---|---|---|---|---|
| Patient 81 | Angina | Cardiology | Male | 54 | hypertension | diabetes | Insulin, antihypertensive | | | severe squeezing or crushing chest pain<br>shortness of breath<br>chest pressure | cough \| NO<br>nausea or vomiting \| NO<br>pain radiates to jaw neck back or shoulders \| YES<br>chest pain worsened by exercise \| YES<br>dizziness \| YES<br>swelling of hands and feet \| NO<br>back pain \| NO<br>neck pain \| NO<br>recurrent infections \| NO<br>restless legs syndrome \| NO<br>rapid heartbeat \| YES<br>chest pressure \| YES<br>rapid heartbeat \| NO<br>arm pain or discomfort \| YES<br>cough with phlegm \| NO |
| Patient 82 | Angina | Cardiology | Male | 47 | diabetes | | | | | squeezing or aching sensation in your chest<br>or arms that may spread to your neck jaw or back<br>shortness of breath<br>weakness | swelling \| NO<br>swelling in your legs ankles or feet \| NO<br>swelling in extremities \| NO<br>cough \| NO<br>fainting \| NO<br>spitting up of food from the esophagus or<br>stomach without nausea \| NO<br>low blood pressure \| NO<br>lesion \| NO<br>chest pressure \| NO<br>depression \| YES<br>sadness \| NO<br>back pain \| NO<br>malnutrition \| NO<br>arm pain or discomfort \| YES<br>cough with phlegm \| NO |
| Patient 87 | Stroke | Neuromedicine \|<br>Medicine / General Physician | Male | 70 | | hypertension | Antihypertensive | | History of stroke | speak in short or incomplete sentence<br>speak unrecognizable words<br>weakness | memory loss \| NO<br>problems with coordination \| YES<br>hoarseness \| NO<br>slurred speech \| NO<br>problems with coordination \| YES<br>weakness of one side of the body \| NO<br>loss of ability to do everyday tasks \| NO<br>substitute one word for another or one sound<br>for another \| NO<br>arm pain or discomfort \| YES<br>cough with phlegm \| NO |
| Patient 88 | Stroke | Neuromedicine \|<br>Medicine / General Physician | Male | 65 | heart_disease | | | | | difficulty understanding<br>difficulty speaking | excess urination \| NO<br>sudden paralysis numbness and weakness in<br>face arm or leg often one side of the body \| NO<br>hoarseness of voice \| NO<br>speak in short or incomplete sentence \| YES<br>weakness \| YES<br>speak unrecognizable words \| NO<br>problems with coordination \| NO<br>confusion \| NO<br>slurred speech \| NO<br>numbness in part of your body \| NO<br>throbbing headache \| NO<br>seizures \| NO<br>weakness of one side of the body \| NO<br>blurred vision \| NO<br>malnutrition \| NO |
| Patient 92 | Sleep apnea | Neuromedicine \|<br>Medicine / General Physician | Male | 32 | | | | | | morning headache<br>sleepiness<br>snoring | constant tiredness \| YES<br>low energy \| YES<br>anxiety \| NO<br>irritability \| YES<br>poor appetite \| YES<br>slow thinking or speech \| YES<br>difficulty remembering \| YES<br>restlessness \| YES |
| Patient 93 | Sleep apnea | Neuromedicine \|<br>Medicine / General Physician | Female | 44 | | | | food | | tiredness or fatigue<br>sleepiness<br>snoring | constant tiredness \| YES<br>low energy \| YES<br>anxiety \| YES<br>irritability \| YES |

# Supplementary Table 4

| | | | | | | | | | | | |
|---|---|---|---|---|---|---|---|---|---|---|---|
| Patient 97 | Arthritis | Rheumatology | Female | 50 | renal disease | | | | History of menopause<br>3 years back | ankle pain<br>swelling<br>stiffness | small red lump on skin \| NO<br>itchy skin \| NO<br>seizures \| NO<br>blistering \| NO<br>joint pain \| YES<br>warm red skin over the affected joint \| YES<br>tenderness in joint \| YES<br>redness in joint \| YES<br>swollen or inflamed joint \| YES<br>knee pain \| YES<br>hip pain \| NO<br>shoulder pain \| NO<br>fever \| NO<br>back pain \| NO<br>leg pain \| YES |
| Patient 98 | Arthritis | Rheumatology | Male | 44 | | | | | | joint pain<br>tenderness in joint<br>stiffness | warm red skin over the affected joint \| YES<br>redness in joint \| YES<br>swollen or inflamed joint \| YES<br>knee pain \| YES<br>hip pain \| YES<br>shoulder pain \| YES |
| Patient 101 | Atrial fibrillation | Cardiology | Male | 56 | heart_disease | | | | | dizziness<br>chest pain<br>shortness of breath | heart palpitations \| YES<br>tiredness or fatigue \| YES<br>swelling of hands and feet \| YES<br>back pain \| YES<br>neck pain \| NO<br>recurrent infections \| NO<br>restless legs syndrome \| NO<br>tiredness or fatigue \| YES<br>wheezing \| NO<br>cough \| NO<br>respiratory distress \| YES<br>rapid heartbeat \| YES<br>chest pressure \| YES<br>low blood pressure \| NO<br>fainting \| NO |
| Patient 102 | Atrial fibrillation | Cardiology | Female | 78 | | hypertension | | | History of taking<br>medicine irregular | lightheadedness<br>chest pressure<br>heart palpitations | dizziness \| YES<br>lethargy \| YES<br>chest pain \| YES<br>tiredness or fatigue \| YES<br>confusion \| YES |
| Patient 106 | Heart failure | Cardiology | Male | 56 | heart_disease | | | Food | | tiredness or fatigue<br>difficulty breathing<br>cough | wheezing \| NO<br>shortness of breath at rest \| YES<br>chest pressure \| YES<br>cough with phlegm \| YES<br>chills or shiver \| NO<br>swelling in your legs ankles or feet \| YES<br>fever \| NO<br>anxiety \| NO<br>depression \| YES<br>sadness \| YES<br>sore throat \| NO<br>nasal congestion \| NO<br>throbbing headache \| NO<br>weight gain \| NO<br>rapid heartbeat \| YES |
| Patient 107 | Heart disease | Cardiology | Female | 45 | | | | | | shortness of breath<br>chest pressure<br>heart palpitations | cough \| YES<br>chest pain \| YES<br>rapid heartbeat \| YES<br>low blood pressure \| YES<br>fainting \| NO<br>lightheadedness \| YES<br>dizziness \| YES<br>lethargy \| YES<br>tiredness or fatigue \| YES |

# Supplementary Table 4

| | | | | | | | | | | | |
|---|---|---|---|---|---|---|---|---|---|---|---|
| Patient 111 | Radiculopathy | Neuromedicine / Orthopedic | Male | 56 | | | | | | weakness in the hands or legs<br>numbness and tingling of the hands<br>weakness | speak in short or incomplete sentence \| NO<br>stiffness or pain in the neck \| NO<br>fainting \| NO<br>excess urination \| NO<br>cloudy or bloody urine \| NO<br>thirst \| NO<br>shakiness \| NO<br>arm pain or discomfort \| YES<br>muscle pain \| YES<br>swelling in the affected area \| NO<br>cramping \| NO<br>leg pain \| YES<br>falling \| NO<br>numbness in part of your body \| YES<br>shoulder pain \| YES |
| Patient 112 | Radiculopathy | Neuromedicine \| Orthopedic | Female | 65 | | | | | | tingling<br>weakness numbness in arms<br>hands or fingers<br>numbness in arm | joint pain \| YES<br>back pain \| YES<br>tenderness in joint \| NO<br>redness in joint \| NO<br>swollen or inflamed joint \| NO<br>knee pain \| NO<br>swelling in the affected area \| NO<br>sudden paralysis numbness and weakness in<br>face arm or leg often one side of the body \| YES<br>severe headache \| NO<br>slurred speech \| NO<br>nausea and vomiting \| NO<br>seizures \| NO<br>sudden vision loss \| NO<br>falling \| NO<br>sudden confusion \| NO |
| Patient 118 | Mosquito borne dis | Medicine / General Physician | Female | 35 | renal disease | | | | | high fever<br>severe acute stabbing muscle pain<br>joint pain | warm red skin over the affected joint \| NO<br>tenderness in joint \| NO<br>skin rash \| YES<br>stiffness in multiple joints \| NO<br>yellow skin and eyes \| NO<br>muscle spasms and pain \| YES<br>cough with phlegm \| NO<br>runny nose \| NO<br>dry cough \| NO<br>sore throat \| NO<br>headache \| YES<br>body ache \| YES<br>tiredness or fatigue \| YES<br>difficulty sleeping \| YES<br>poor appetite \| YES |
| Patient 125 | Arthritis | Rheumatology | Male | 50 | diabetes | | | | History of taking<br>alcohol | intense joint pain usually at big toe<br>stiffness in joint especially in the morning<br>redness in joint | tingling pain or numbness in the hands and feet \| YES<br>swelling in the affected area \| YES<br>hand joints are warm and tender to the touch \| YES<br>fever \| NO<br>knee pain \| YES<br>recurrent infections \| NO<br>acute episodes \| YES<br>weakness \| NO<br>shortness of breath at rest \| NO<br>diarrhoea \| NO<br>shoulder pain \| NO<br>redness in the affected area \| YES<br>tiredness or fatigue \| YES<br>hip pain \| NO<br>depression \| NO |
| Patient 126 | Kidney disease | Nephrology | Male | 54 | diabetes | diabetes,hypertension | Insulin | | | swollen ankles feet or hands<br>cloudy or bloody urine<br>dry skin | yellow skin and eyes \| NO<br>high blood pressure \| YES<br>blurred vision \| NO<br>urinating more or less than normal \| YES<br>protein in the urine \| YES<br>shortness of breath \| YES<br>severe headache \| NO<br>pain in upper abdomen \| NO<br>weight loss \| YES<br>puffy eyes \| YES<br>sudden vision loss \| NO<br>sensitivity to light \| NO<br>pain under the ribs on the right side \| NO |

Supplementary Table 4

| | | | | | | | | | | | |
|---|---|---|---|---|---|---|---|---|---|---|---|
| Patient 131 | Chronic obstructive pulmonary disease | Respiratory / Chest Disease | Male | 45 | COPD | | | | History of smoking | cough with phlegm<br>persistent cough<br>shortness of breath | fever \| NO<br>recurring chest infection \| YES<br>chest pressure \| YES<br>sore throat \| NO<br>shortness of breath at rest \| YES<br>weight gain \| NO<br>fluid in the lungs \| NO<br>blue or gray skin color due to low oxygen levels \| YES<br>lethargy \| YES<br>difficulty breathing \| YES<br>tiredness or fatigue \| YES<br>respiratory distress \| YES<br>rapid breathing \| YES<br>swelling in extremities \| NO |
| Patient 132 | Asthma | Respiratory / Chest Disease | Female | 48 | asthma | | | | | wheezing<br>sudden high fever<br>shortness of breath | swelling in the affected area \| YES<br>cough \| YES<br>weight gain \| NO<br>fluid in the lungs \| YES<br>blue or gray skin color due to low oxygen levels \| YES<br>increased heart rate \| YES<br>fainting \| NO<br>shortness of breath at rest \| YES<br>cough with phlegm \| YES<br>persistent wheezing \| YES |
| Patient 137 | Heart failure | Cardiology | Female | 55 | heart_disease | hypertension | Antihypertensive | | | shortness of breath with activity or when lying down<br>swelling in leg or ankle<br>rapid heartbeat | persistent cough \| YES<br>chest pain \| YES<br>heart palpitations \| YES<br>chest pressure \| YES<br>low blood pressure \| NO<br>fainting \| NO<br>lightheadedness \| YES<br>dizziness \| YES<br>lethargy \| YES<br>weight gain \| NO<br>tiredness or fatigue \| YES<br>dry cough \| NO<br>anxiety \| YES<br>cavity \| NO<br>chest discomfort \| YES |
| Patient 138 | Heart failure | Cardiology | Male | 49 | | hypertension | Antihypertensive | | History of alcohol abuse | trouble taking deep breath<br>persistent wheezing<br>shortness of breath | heart palpitations \| YES<br>dizziness \| YES<br>chest pain \| YES<br>swelling in your legs ankles or feet \| YES<br>back pain \| NO<br>neck pain \| NO<br>recurrent infections \| NO<br>restless legs syndrome \| NO<br>tiredness or fatigue \| YES<br>respiratory distress \| YES<br>chest discomfort \| YES<br>cavity \| NO<br>malnutrition \| NO<br>dry cough \| NO<br>drooping of upper eyelid \| NO |
| Patient 142 | Inflammatory bowel disease | Gastroenterology | Female | 77 | | | | | | severe pain in abdomen<br>diarrhoea<br>fever | nausea and vomiting \| YES<br>cough with phlegm \| NO<br>runny nose \| NO<br>dry cough \| NO<br>sore throat \| NO<br>headache \| NO<br>muscle pain \| NO<br>body ache \| NO<br>difficulty sleeping \| YES<br>poor appetite \| YES<br>mouth ulcer \| YES<br>acute episodes \| NO<br>blood in stool \| YES<br>diarrhoea with blood or pus \| YES |

# Supplementary Table 4

| | | | | | | | | | | | |
|---|---|---|---|---|---|---|---|---|---|---|---|
| Patient 143 | Inflammatory bowe<br>disease | Gastroenterology | Male | 34 | | | | | | pain in abdomen<br>diarrhoea<br>cramping in abdomen | blood in stool \| YES<br>nausea and vomiting \| NO<br>acute episodes \| NO<br>bleeding from anus \| YES<br>fever \| YES<br>tenderness in the affected area \| YES<br>weight loss \| YES<br>unexplained fatigue \| YES<br>dehydration \| YES<br>bowel obstruction \| YES<br>rectum pain \| YES<br>rapid heartbeat \| NO |
| Patient 151 | Diverticulitis | Gastroenterology | Male | 45 | | | | | | persistent pain in lower left side of the abdomen<br>nausea or vomiting<br>fever | pain in upper-right abdomen that radiates to<br>back and shoulder \| NO<br>mild fever \| YES<br>cough with phlegm \| NO<br>runny nose \| NO<br>dry cough \| NO<br>sore throat \| NO<br>headache \| NO<br>muscle pain \| NO<br>live or travelled recently to areas prone to viral fevers<br>like dengue malaria chikungunya or high prevalence<br>of hepatitis (e.g. India or Africa) \| NO<br>dull pain in upper-right abdomen \| NO<br>poor appetite \| YES<br>yellow skin and eyes \| NO<br>pale stool \| NO<br>high fever \| NO<br>cloudy or bloody urine \| NO |
| Patient 152 | Diverticulitis | Gastroenterology | Female | 65 | | | | | | persistent pain in lower left side of the abdomen<br>nausea and vomiting<br>diarrhoea | pain in upper-right abdomen that radiates to back and<br>shoulder \| NO<br>dull pain in upper-right abdomen \| NO<br>high blood pressure \| NO<br>mild fever \| NO<br>live or travelled recently to areas prone to viral fevers like<br>dengue malaria chikungunya or high prevalence<br>of hepatitis (e.g. India or Africa) \| NO<br>high fever \| NO<br>blood in stool \| YES<br>bleeding from anus \| YES<br>swelling in the face hands or legs \| NO<br>yellow skin and eyes \| NO<br>excess urination \| NO<br>poor appetite \| NO<br>chills or shiver \| YES<br>burning sensation during urination \| NO<br>bulge in the tummy \| NO |
| Patient 157 | Mosquito borne dis | Medicine / General Physician | Male | 22 | | | | | History of travel to<br>hillside | headache<br>chills or shiver<br>fever | urine leakage around your catheter \| NO<br>sudden severe headache \| YES<br>high fever \| YES<br>live or travelled recently to areas prone to viral fevers like<br>dengue malaria chikungunya or high prevalence<br>of hepatitis (e.g. India or Africa) \| YES<br>skin rash \| YES<br>cold hands and feet \| YES<br>excessive sweating \| YES<br>stiffness or pain in the neck \| NO<br>nausea and vomiting \| YES<br>drowsiness \| NO<br>dislike of bright lights \| YES<br>malaise \| YES<br>confusion \| YES<br>joint pain \| YES<br>back pain \| YES |

# Supplementary Table 4

| | | | | | | | | | | | |
|---|---|---|---|---|---|---|---|---|---|---|---|
| Patient 158 | Mosquito borne dis | Medicine / General Physician | Male | 38 | | | | Na | History of travel to hillside | relapsing moderate fever for more than 7 days<br>fever and chills<br>throbbing headache | pain in abdomen \| YES<br>constipation \| NO<br>bleeding from your nose without any injury \| NO<br>throbbing headache \| YES<br>live or travelled recently to areas prone to viral fevers like dengue malaria chikungunya or high prevalence of hepatitis (e.g. India or Africa) \| YES<br>pale or mottled skin \| NO<br>cold hands and feet \| NO<br>skin rash \| YES<br>stiffness or pain in the neck \| NO<br>drowsiness \| YES<br>malaise \| YES<br>chills or shiver \| YES<br>confusion \| YES |
| Patient 161 | Urinary tract infecti | Medicine / General Physician | Female | 25 | | | | | History of getting married recently | burning sensation or pain during urination<br>pain in lower abdomen<br>cloudy or bloody urine | frequent urge to urinate \| YES<br>feeling like you need to pee again soon after going to the toilet \| YES<br>strong urine odor \| YES<br>malaise \| YES<br>tiredness or fatigue \| YES<br>fever \| YES<br>chills or shiver \| YES |
| Patient 162 | Urinary tract infecti | Medicine / General Physician | Female | 18 | | | | | History of getting married recently | fever<br>burning sensation or pain during urination | strong persistent urge to urinate \| YES<br>small amount of urine \| YES<br>pelvic pain \| YES<br>cloudy or bloody urine \| NO<br>pain in lower abdomen \| YES<br>strong urine odor \| YES<br>chills or shiver \| YES |
| Patient 177 | Hypoglycemia | Diabetes / Endocrinology | Male | 50 | hypertension | diabetes | Oral hypoglycaemic agents | | History of missed meal | feeling shaky or trembling<br>dizziness<br>confusion | excess urination \| NO<br>rapid heartbeat \| YES<br>increased hunger \| YES<br>seizures \| NO<br>cuts or infection taking much longer to heal \| YES<br>excess thirst \| YES<br>fever \| NO<br>slurred speech \| YES<br>pale skin \| YES<br>blurred vision \| YES<br>nausea and vomiting \| NO<br>recurrent infections \| YES<br>lethargy \| YES<br>diarrhoea \| NO<br>tiredness or fatigue \| YES |
| Patient 178 | Hypoglycemia | Diabetes / Endocrinology | Male | 39 | | diabetes | Oral hypoglycaemic agents | | History of missed medicine | lightheadedness<br>dizziness<br>rapid heartbeat | loss of coordination and balance \| YES<br>weight loss \| NO<br>low blood pressure \| NO<br>thirst \| YES<br>sweating \| YES<br>excess urination \| NO<br>blurred vision \| NO<br>tingling lips \| YES<br>confusion \| YES<br>feeling cold \| YES |
| Patient 182 | Arthritis | Rheumatology | Male | 74 | renal disease | diabetes | | Food | | stiffness<br>tenderness in joint<br>pain | joint pain \| YES<br>stiffness in multiple joints \| YES<br>swelling in the affected area \| YES<br>fever \| NO<br>knee pain \| YES<br>recurrent infections \| YES<br>acute episodes \| NO<br>weakness \| YES<br>shortness of breath at rest \| NO<br>diarrhoea \| NO<br>shoulder pain \| NO<br>redness in the affected area \| YES<br>tiredness or fatigue \| YES<br>chills or shiver \| NO<br>hip pain \| NO |

# Supplementary Table 4

| | | | | | | | | | | | |
|---|---|---|---|---|---|---|---|---|---|---|---|
| Patient 183 | Arthritis | Rheumatology | Male | 39 | diabetes | diabetes | Insulin | | | stiffness<br>tenderness in the affected area<br>pain | testicle pain \| NO<br>joint pain \| YES<br>tenderness in joint \| YES<br>stiffness in multiple joints \| YES<br>swelling in the affected area \| YES<br>fever \| NO<br>knee pain \| NO<br>recurrent infections \| NO<br>acute episodes \| NO<br>weakness \| NO<br>shortness of breath at rest \| NO<br>diarrhoea \| NO<br>redness in the affected area \| YES<br>tiredness or fatigue \| YES |
| Patient 191 | Irritable bowel syndrome | Gastroenterology | Male | 29 | | | | | | cramping<br>diarrhoea<br>discomfort in abdomen | pain in abdomen \| YES<br>blood in stool \| NO<br>nausea and vomiting \| NO<br>acute episodes \| NO<br>yellow skin and eyes \| NO<br>diarrhoea with blood or pus \| NO<br>bleeding from anus \| NO<br>food intolerance \| YES<br>swelling in abdomen \| YES<br>pain relieved after bowel movement \| YES<br>gas \| YES<br>constipation \| YES<br>belching \| YES<br>anxiety \| NO<br>pain in lower abdomen \| YES |
| Patient 192 | Irritable bowel syndrome | Gastroenterology | Male | 44 | diabetes | | | | | constipation or diarrhoea<br>diarrhoea<br>discomfort in abdomen | pain in abdomen \| YES<br>food intolerance \| YES<br>nausea and vomiting \| NO<br>bloating \| YES<br>pain relieved after bowel movement \| YES<br>gas \| NO<br>cramping \| YES<br>belching \| NO<br>anxiety \| YES<br>pain in lower abdomen \| YES<br>acute episodes \| NO<br>poor appetite \| NO<br>rectum pain \| NO<br>dehydration \| YES<br>tenderness in the affected area \| NO |
| Patient 201 | Kidney stone | Urologist | Male | 29 | | | | Dust | | pain during urination<br>pain in the back belly or side more than a week<br>cloudy or bloody urine | high blood pressure \| NO<br>frequent urge to urinate \| YES<br>fever and chills \| YES<br>redness in joint \| NO<br>belching \| NO<br>tenderness in joint \| NO<br>nausea and vomiting \| YES<br>diarrhoea \| NO<br>blood in stool \| NO<br>testicle pain \| NO<br>pain in upper abdomen \| NO<br>rectum pain \| NO<br>swollen or inflamed joint \| NO<br>increased size of your abdomen due to enlarged kidneys \| NO<br>cramping \| YES |
| Patient 202 | Kidney stone | Urologist | Female | 33 | diabetes | | | | | flank pain<br>cloudy or bloody urine<br>pain during urination | high blood pressure \| NO<br>groin pain \| YES<br>joint pain \| NO<br>diarrhoea \| NO<br>irregular heartbeat \| NO<br>frequent urge to urinate \| YES<br>tissue fragment in urine \| YES<br>fever and chills \| YES<br>swelling in your legs ankles or feet \| NO<br>pain in the back belly or side more than a week \| YES |
| Patient 206 | Meningitis | Neuromedicine | Male | 39 | | | | | | headache<br>high fever<br>stiffness or pain in the neck | sudden severe headache \| YES<br>live or travelled recently to areas prone to diseases like meningitis (e.g. sub-Saharan Africa) \| YES<br>pale or mottled skin \| YES<br>cold hands and feet \| YES<br>skin rash \| YES<br>nausea and vomiting \| YES |

# Supplementary Table 4

| | | | | | | | | | | | |
|---|---|---|---|---|---|---|---|---|---|---|---|
| Patient 207 | Meningitis | Neuromedicine | Male | 45 | diabetes | diabetes | Insulin | Dust | | high fever<br>stiffness or pain in the neck<br>nausea and vomiting | live or travelled recently to areas prone to viral fevers like dengue malaria chikungunya or high prevalence of hepatitis (e.g. India or Africa) \| NO<br>headache \| YES<br>sudden severe headache \| YES<br>live or travelled recently to areas prone to diseases like meningitis (e.g. sub-Saharan Africa) \| YES<br>pale or mottled skin \| NO<br>cold hands and feet \| YES<br>skin rash \| YES<br>drowsiness \| YES<br>dislike of bright lights \| YES<br>malaise \| YES<br>chills or shiver \| YES<br>confusion \| YES<br>joint and muscle pain \| NO<br>back pain \| YES<br>lethargy \| YES |
| Patient 217 | Osteoporosis | Rheumatology | female | 55 | heart_disease | | | | | stooped posture<br>back pain<br>loss of height over time | bone breaks much more easily than expected \| YES<br>pain increases with movement \| YES<br>depression \| YES<br>sadness \| YES<br>hip pain \| YES |
| Patient 218 | Osteoporosis | Rheumatology | Female | 50 | | | | | | bone breaks much more easily than expected<br>back pain<br>stooped posture | pain worsen by moving and relieved when lie down \| YES<br>loss of height over time \| YES<br>depression \| YES<br>sadness \| YES<br>hip pain \| YES |
| Patient 226 | Gout | Rheumatology | Male | 34 | | | | | | sudden severe acute pain at big toe<br>swelling at big toe<br>difficulty walking | sudden attack of pain \| YES<br>warm red skin over the affected joint \| YES<br>redness in the affected joint \| YES<br>swollen or inflamed joint \| YES<br>knee pain \| NO<br>stiffness \| NO<br>hip pain \| NO<br>shoulder pain \| NO<br>fever \| NO<br>back pain \| NO<br>leg pain \| NO<br>recurrent infections \| NO<br>arm pain or discomfort \| NO<br>foot pain \| YES<br>depression or irritability \| YES |
| Patient 227 | Gout | Rheumatology | Male | 44 | renal disease | diabetes | Insulin | | | severe pain<br>redness in the affected joint<br>swollen or inflamed joint | intense joint pain usually at big toe \| YES<br>warm red skin over the affected joint \| YES<br>redness in joint \| YES<br>tenderness in joint \| YES<br>knee pain \| YES<br>swelling in the affected area \| YES<br>stiffness \| YES<br>hip pain \| YES<br>shoulder pain \| YES<br>fever \| YES<br>back pain \| NO<br>leg pain \| NO<br>stiffness or pain in the neck \| NO<br>recurrent infections \| YES<br>arm pain or discomfort \| YES |
| Patient 231 | Heart failure | Cardiology | Male | 39 | | | | | | shortness of breath<br>heart palpitations<br>swollen ankles feet or hands | cough \| YES<br>shortness of breath or chest pain or palpitation worsen when lying down \| YES<br>weight gain \| NO<br>fluid in the lungs \| NO<br>wheezing \| NO<br>blue or gray skin color due to low oxygen levels \| YES<br>cough with phlegm \| NO<br>dry cough \| YES<br>chest pain \| YES<br>difficulty breathing \| YES<br>chest pressure \| YES<br>tiredness or fatigue \| YES<br>respiratory distress \| YES<br>rapid breathing \| YES<br>swelling in extremities \| YES |

# Supplementary Table 4

| | | | | | | | | | | | |
|---|---|---|---|---|---|---|---|---|---|---|---|
| Patient 232 | Heart failure | Cardiology | Male | 43 | asthma | | | | | tiredness or fatigue<br>chest pain<br>shortness of breath | swelling in your legs ankles or feet | YES<br>cough | YES<br>dizziness | YES<br>fainting | YES<br>lightheadedness | YES<br>spitting up of food from the esophagus or stomach without nausea | NO<br>lethargy | YES<br>weight gain | YES<br>tiredness or fatigue | YES<br>dry cough | YES<br>anxiety | YES<br>chest discomfort | YES |
| Patient 237 | Embolism | Medicine / General Physician | Male | 55 | heart_disease | | | | | chest pain<br>sudden shortness of breath<br>irregular heartbeat | sharp chest pain that worsen by breathing | YES<br>coughing up blood | NO<br>rapid heartbeat | YES<br>swelling in leg or ankle | YES<br>fever | NO<br>clammy skin | YES<br>low oxygen in the body | NO<br>excessive sweating | YES<br>discomfort | YES<br>calf pain | NO<br>blue skin or lips | NO<br>dizziness | YES<br>recurrent infections | NO<br>chest discomfort | YES<br>leg pain | YES |
| Patient 238 | Embolism | Medicine / General Physician | Male | 48 | | hypertension | Anti hypertensive | | | chest pain<br>anxiety<br>sudden shortness of breath | sharp chest pain that worsen by breathing | YES<br>coughing up blood | NO<br>rapid breathing | YES<br>swelling in your legs ankles or feet | YES<br>fever | NO<br>clammy or discolored skin | NO<br>low oxygen in the body | NO<br>excessive sweating | YES<br>discomfort in abdomen | NO<br>calf pain | NO<br>blue skin or lips | NO<br>dizziness | YES<br>recurrent infections | YES<br>chest discomfort | YES<br>leg pain | NO |
| Patient 242 | Tuberculosis | Medicine / General Physician | Male | 44 | renal disease | | | | | night sweat<br>fever and chills<br>mild cough | persistent cough | YES<br>coughing up blood | NO<br>cough with phlegm | NO<br>live or travelled recently to areas prone to viral fevers like dengue malaria chikungunya or high prevalence of hepatitis (e.g. India or Africa) | NO<br>tiredness or fatigue | YES<br>evening rise of temperature | YES<br>weight loss | YES<br>persistent fever | YES<br>poor appetite | YES<br>shortness of breath | NO<br>chills or shiver | YES<br>pale or bluish skin | NO<br>nausea and vomiting | YES<br>wheezing | NO<br>rapid breathing | NO |
| Patient 243 | Tuberculosis | Medicine / General Physician | Male | 29 | | | | | | night sweat<br>fever and chills<br>cough | persistent cough | YES<br>coughing up blood | NO<br>cough with phlegm | NO<br>live or travelled recently to areas prone to viral fevers like dengue malaria chikungunya or high prevalence of hepatitis (e.g. India or Africa) | NO<br>tiredness or fatigue | YES<br>evening rise of temperature | YES<br>weight loss | YES<br>persistent fever | YES<br>poor appetite | YES<br>shortness of breath | YES<br>chills or shiver | YES<br>pale or bluish skin | YES<br>nausea and vomiting | YES<br>wheezing | YES<br>rapid breathing | NO |

# Supplementary Table 4

| | | | | | | | | | | | |
|---|---|---|---|---|---|---|---|---|---|---|---|
| Patient 252 | Retinopathy | Nephrology | Male | 38 | diabetes | diabetes,hypertension | Insulin, anti hypertensive | | | blurred vision<br>excess urination<br>excess thirst | shapes in vision \| YES<br>weight loss \| NO<br>fluctuating vision \| NO<br>gradual worsening of vision \| YES<br>sudden vision loss \| YES<br>fever \| NO<br>impaired color vision \| NO<br>nausea or vomiting \| NO<br>recurrent infections \| YES<br>lethargy \| YES<br>diarrhoea \| NO<br>tiredness or fatigue \| YES<br>dizziness \| YES<br>pain during urination \| NO<br>shortness of breath \| NO |
| Patient 253 | Renal disroder | Nephrology | Male | 55 | diabetes,diab | diabetes | Insulin | Dust | | excess urination<br>excess thirst<br>tiredness or fatigue | weight loss \| YES<br>excess mucus \| YES<br>cuts or infection taking much longer to heal \| YES<br>fever \| NO<br>tiredness or fatigue \| YES<br>blurred vision \| YES<br>nausea or vomiting \| NO<br>recurrent infections \| YES<br>lethargy \| YES<br>diarrhoea \| YES<br>dizziness \| YES<br>pain during urination \| NO<br>shortness of breath \| NO<br>foot pain \| NO<br>cough \| NO |
| Patient 262 | Arthritis | Rheumatology | Female | 25 | asthma | | | | | tenderness in the affected area<br>stiffness in joint especially in the morning<br>tiredness or fatigue | tingling pain or numbness in the hands and feet \| YES<br>swelling in the affected area \| YES<br>warm red skin over the affected joint \| YES<br>fever \| NO<br>knee pain \| YES<br>joint pain \| YES<br>recurrent infections \| NO<br>acute episodes \| NO<br>weakness \| YES<br>shortness of breath at rest \| NO<br>diarrhoea \| NO<br>shoulder pain \| YES<br>redness in the affected area \| YES<br>tiredness or fatigue \| YES<br>hip pain \| YES |
| Patient 263 | Arthritis | Rheumatology | Female | 32 | | | | Dust | | tenderness in the affected area<br>redness in the affected joint<br>stiffness in multiple joints | pain \| YES<br>joint pain \| YES<br>tenderness in joint \| YES<br>swelling in the affected area \| YES<br>fever \| NO<br>knee pain \| NO<br>recurrent infections \| NO<br>acute episodes \| NO<br>weakness \| NO<br>shortness of breath at rest \| NO<br>diarrhoea \| NO<br>shoulder pain \| NO<br>redness in the affected area \| YES<br>tiredness or fatigue \| YES<br>hip pain \| NO |
| Patient 267 | Stroke | Neuromedicine | Male | 27 | asthma | | | | | blurred vision<br>sudden confusion<br>sudden numbness | sudden paralysis numbness and weakness in<br>face arm or leg often one side of the body \| YES<br>slurred speech \| YES<br>severe headache \| YES<br>sudden vision loss \| YES<br>falling \| YES<br>problem with balance or coordination \| YES<br>dizziness \| YES |
| Patient 268 | Stroke | Neuromedicine | Male | 43 | | hypertension | Anti hypertensive | | | sudden vision loss<br>sudden severe headache<br>slurred speech | sudden paralysis numbness and weakness in<br>face arm or leg often one side of the body \| YES<br>sudden numbness \| YES<br>falling \| YES<br>sudden confusion \| YES<br>blurred vision \| YES<br>problem with balance or coordination \| YES<br>dizziness \| YES<br>numbness in arm \| YES<br>sudden weakness \| YES |

# Supplementary Table 4

| | | | | | | | | | | | |
|---|---|---|---|---|---|---|---|---|---|---|---|
| Patient 277 | Inflammatory bowe<br>disease | Gastroenterology | Female | 38 | heart_disease | | | | | blood in stool<br>diarrhoea with blood or pus<br>moderate chronic pain in abdomen for a few days to w | bleeding from anus \| YES<br>feel like you still need to poo after going to the toilet \| YES<br>constipation \| NO<br>mucus in your underwear or on toilet paper<br>after wiping your bottom \| YES<br>pain during defecation \| YES<br>pain around anus \| YES<br>weight loss \| YES<br>belching \| NO |
| Patient 278 | Inflammatory bowe<br>disease | Gastroenterology | Female | 49 | asthma | | | | | blood in stool<br>pain in abdomen<br>diarrhoea | nausea or vomiting \| NO<br>acute episodes \| YES<br>bleeding from anus \| YES<br>fever \| NO<br>tenderness in the affected area \| NO<br>pain in lower abdomen \| YES<br>scarring within the bile ducts \| NO<br>weight loss \| NO<br>tiredness or fatigue \| YES<br>lethargy \| YES<br>dehydration \| NO<br>bowel obstruction \| YES<br>rectum pain \| YES<br>diarrhoea with blood or pus \| YES<br>rapid heartbeat \| NO |
| Patient 282 | Diabetes mellitus | Diabetes / Endocrinology | Female | 20 | | | | | | blurred vision<br>excess urination<br>excess thirst | shapes in vision \| NO<br>weight loss \| NO<br>excess night urination \| YES<br>cuts or infection taking much longer to heal \| YES<br>fever \| NO<br>nausea or vomiting \| NO<br>recurrent infections \| YES<br>chills or shiver \| NO<br>lethargy \| YES<br>diarrhoea \| NO<br>tiredness or fatigue \| YES<br>increased hunger \| YES<br>foot ulcer \| YES<br>odors from the affected area \| YES<br>dizziness \| YES |
| Patient 283 | Diabetes mellitus | Diabetes / Endocrinology | Male | 19 | diabetes | | | | | blurred vision<br>excess thirst<br>excess urination | shapes in vision \| NO<br>weight loss \| YES<br>excess urination \| YES<br>cuts or infection taking much longer to heal \| YES<br>fever \| NO<br>tiredness or fatigue \| YES<br>increased hunger \| YES<br>foot ulcer \| YES<br>odors from the affected area \| YES<br>nausea and vomiting \| NO<br>recurrent infections \| YES<br>lethargy \| YES<br>diarrhoea \| NO<br>dizziness \| YES<br>pain during urination \| YES |
| Patient 290 | Stroke | Neuromedicine \|<br>Medicine / General Physician | Male | 73 | hypertension | hypertension | Anti hypertensive | | | sudden paralysis numbness and weakness in face arm<br>slurred speech<br>sudden confusion | nausea and vomiting \| YES<br>blurred vision \| YES<br>sweating \| NO<br>numbness in part of your body \| YES<br>poor concentration \| YES<br>one side of the face drooling \| YES<br>depression \| NO<br>agitation \| NO<br>seizures \| NO<br>fainting \| YES<br>agitation \| YES<br>hip pain \| YES<br>lethargy \| YES |
| Patient 291 | Stroke | Neuromedicine \|<br>Medicine / General Physician | Female | 59 | | hypertension | Anti hypertensive | | | blurred vision<br>difficulty speaking<br>sudden numbness | sudden paralysis numbness and weakness in<br>face arm or leg often one side of the body \| YES<br>slurred speech \| YES<br>headache \| YES<br>sudden vision loss \| YES<br>falling \| YES<br>sudden confusion \| YES<br>problem with balance or coordination \| YES<br>dizziness \| YES |

# Supplementary Table 4

| | | | | | | | | | | | |
|---|---|---|---|---|---|---|---|---|---|---|---|
| Patient 297 | Eczema | Skin / Dermatology | Male | 30 | diabetes | | | | | dry skin<br>itching<br>skin rash | lice on head \| NO<br>small red lump on skin \| NO<br>cracked or scaly skin \| YES<br>bumps and blisters on skin \| YES<br>oozing on skin \| YES<br>crusting of the skin \| YES<br>thickened skin in the affected area \| YES |
| Patient 298 | Eczema | Skin / Dermatology | Female | 37 | | diabetes | Insulin | | | itchy skin<br>dry cracked skin<br>oozing on skin | purple rashes on brown skin or pink or red rash<br>on white skin \| YES<br>dry and cracked skin that may bleed \| YES<br>itchy skin \| YES<br>bleeding from scratched skin \| YES<br>scaly plaques on the skin \| YES<br>soreness in skin \| YES |
| Patient 302 | Athlete's foot | Medicine / General Physician | Female | 55 | diabetes | | | | | inflamed skin that might appear reddish purplish or gra<br>blistering<br>itching between toes | cracked skin between the toes \| YES<br>white patches between your toes \| YES<br>dry scaly skin on the bottom of the foot that extends<br>up the side \| YES<br>blisters between toes \| YES<br>sweating \| NO<br>itchiness especially right after taking off shoes and socks \| YES<br>burning in feet and toes \| YES<br>frequently wear enclosed footwear \| YES |
| Patient 303 | Athlete's foot | Medicine / General Physician | Male | 38 | diabetes | | | | | blisters between toes<br>itching between toes<br>cracked or scaly skin | cracked skin between the toes \| YES<br>white patches between your toes \| YES<br>dry scaly skin on the bottom of the foot that extends<br>up the side \| YES<br>sweating \| YES<br>itchiness especially right after taking off shoes and socks \| YES |
| Patient 307 | Flu | Medicine / General Physician | Female | 28 | | | | | | malaise<br>runny nose<br>fever | sore throat \| YES<br>cough \| YES<br>nasal congestion \| YES<br>body ache \| YES<br>mild headache \| YES |
| Patient 308 | Flu | Medicine / General Physician | Male | 44 | | hypertension | Anti hypertensive | | | runny nose<br>sore throat<br>fever | cough \| YES<br>nasal congestion \| YES<br>slight body ache \| YES<br>mild headache \| YES |
| Patient 316 | Constipation | Medicine / General Physician | Male | 44 | diabetes | | | Food | | lumpy or hard stools<br>passing fewer than three stools a week | difficulty in bowel movement \| YES<br>a feeling as though you can't completely empty<br>the stool from your rectum \| YES<br>a feeling as though there is a blockage in your<br>rectum that prevents bowel movements \| YES<br>dehydration \| YES<br>little or no physical activity \| YES |
| Patient 317 | Constipation | Medicine / General Physician | Male | 59 | | | | | | lumpy or hard stools<br>passing fewer than three stools a week | difficulty in bowel movement \| YES<br>a feeling as though you can't completely empty<br>the stool from your rectum \| YES<br>a feeling as though there is a blockage in your<br>rectum that prevents bowel movements \| YES<br>dehydration \| YES<br>little or no physical activity \| YES |
| Patient 322 | Thread worms | Medicine / General Physician | Female | 47 | diabetes | | | N\A | | poor appetite<br>weight loss<br>itching in anus | sudden bed wetting for children \| YES<br>weight loss \| YES<br>itching around the genitals \| YES |
| Patient 323 | Thread worms | Medicine / General Physician | Female | 32 | | | | N\A | | itching in anus<br>itching around vagina | redness and sometimes infection around the anal area \| YES<br>blood in stool \| NO<br>feel like you still need to poo after going to the toilet \| NO<br>pain around anus \| NO<br>trouble sleeping because of the itchiness in anus \| YES<br>weight loss \| DO NOT KNOW |
| Patient 362 | Cystitis | Medicine / General Physician | Female | 23 | | | | N\A | | pain in lower abdomen<br>strong persistent urge to urinate | burning sensation or pain during urination \| YES<br>excess urination \| NO<br>cloudy urine \| YES<br>hectic high fever for more than 7 days \| YES<br>back pain \| NO<br>nausea or vomiting \| NO<br>blood in urine \| YES<br>cloudy urine \| YES<br>malaise \| YES<br>smelly urine \| YES |
| Patient 363 | Pelvic inflammatory<br>disease | Gynaecology | Female | 28 | | | | N\A | | abnormal vaginal bleeding<br>pain in lower abdomen<br>pain during or after sex | urine retention \| NO<br>urine leakage \| NO<br>abnormal vaginal discharge \| YES<br>itching and irritation or fissure around the vagina \| YES |

# Supplementary Table 4

| | | | | | | | | | | | |
|---|---|---|---|---|---|---|---|---|---|---|---|
| Patient 374 | Fungal infection | Medicine / General Physician | Male | 65 | diabetes | | | | | loss of taste<br>creamy white lesions on tongue | slightly raised lesions with a cottage cheese like appearance \| YES<br>a painful burning sensation in the mouth \| YES<br>redness \| NO<br>slight bleeding if the lesions are rubbed or scraped \| YES |
| Patient 375 | Fungal infection | Medicine / General Physician | Female | 33 | diabetes | | | | | abnormal vaginal discharge<br>itching and irritation or fissure around the vagina | pain during urination \| YES<br>abnormal vaginal discharge \| YES |
| Patient 382 | Piles | Medicine / General Physician | Male | 45 | | | | | | blood in stool<br>lump around anus | itching in anus \| YES<br>still need to poo after going to the toilet \| YES<br>mucus in your underwear or on toilet paper<br>after wiping your bottom \| YES |
| Patient 383 | Piles | Medicine / General Physician | Male | 39 | | | | | | blood in stool<br>itching in anus | still need to poo after going to the toilet \| YES<br>mucus in your underwear or on toilet paper after wiping<br>your bottom \| YES |
| Patient 393 | Costochondritis | Medicine / General Physician | Male | 45 | | | | | | pain on the left side of your chest bone or ribs<br>chest pain in multiple chest bones or ribs<br>chest pain when you cough | sharp aching or pressure like pain in chest bones or ribs \| YES<br>chest pain that radiates to arms and shoulders \| YES<br>chest pain \| YES<br>chest pain when you press on chest bone or ribs \| YES<br>chest pain when you cough \| YES |
| Patient 394 | Costochondritis | Medicine / General Physician | Female | 30 | | | | | | pain on the left side of your chest bone or ribs<br>pain radiates to jaw neck back or shoulders<br>high fever | sharp aching or pressure like pain in chest bones or ribs \| YES<br>chest pain in multiple chest bones or ribs \| YES<br>chest pain when you press on chest bone or ribs \| YES<br>chest pain when you cough \| YES |
| Patient 395 | Hepatitis | Hepatology | Male | 39 | | | | | | yellow skin and eyes<br>light color stool<br>nausea and vomiting | malaise \| YES<br>live or travelled recently to areas prone to viral fevers<br>like dengue malaria chikungunya or high prevalence<br>of hepatitis (e.g. India or Africa) \| NO<br>mild fever \| YES<br>pain in upper abdomen \| YES<br>light clay-colored stool \| YES<br>diarrhoea \| NO<br>constipation \| NO<br>cloudy or bloody urine \| NO<br>headache in forehead \| NO<br>muscle pain \| NO<br>tiredness or fatigue \| YES<br>itchy skin \| YES<br>bleeding easily \| NO |
| Patient 396 | Hepatitis | Hepatology | Female | 40 | | | | | | yellow skin and eyes<br>poor appetite<br>pain in abdomen | vomiting \| YES<br>pain in upper abdomen \| YES<br>belching \| NO<br>dark urine \| YES<br>burning in your abdomen \| NO<br>live or travelled recently to areas prone to diseases<br>like meningitis (e.g. sub-Saharan Africa) \| NO<br>bloating \| NO<br>pain in upper-right abdomen that radiates to back and<br>shoulder \| NO<br>diarrhoea \| NO<br>constipation \| NO<br>pain in upper abdomen \| YES<br>cramping \| NO<br>tenderness in abdomen \| NO<br>joint pain \| YES |
| Patient 397 | Scabies | Skin / Dermatology | Male | 35 | | | | | | itching worse at night<br>skin rash<br>itchy skin | thin wavy tunnels made up of tiny blisters or bumps<br>on the skin \| NO<br>itching between the fingers and toes \| NO<br>dry skin \| YES<br>cracked or scaly skin \| NO<br>bumps and blisters on skin \| YES<br>oozing \| NO<br>crusting \| NO<br>thickened skin \| YES |
| Patient 398 | Scabies | Skin / Dermatology | Male | 21 | | | | | | itchy skin<br>itching worse at night<br>an itchy rash on your skin | thin wavy tunnels made up of tiny blisters or bumps<br>on the skin \| YES<br>itching between the fingers and toes \| YES<br>itching in the groin area \| YES<br>dry skin \| YES<br>cracked or scaly skin \| NO<br>bumps and blisters on skin \| YES<br>oozing \| NO<br>crusting \| NO<br>thickened skin \| YES<br>itching around the genitals \| YES<br>scaly patches of skin \| YES |

# Supplementary Table 4

| | | | | | | | | | | | |
|---|---|---|---|---|---|---|---|---|---|---|---|
| Patient 399 | Heart disease | Cardiology | Male | 56 | hypertension | | | | | squeezing or aching sensation in your chest or arms th<br>chest pressure<br>severe acute crushing chest pain that occurs at rest typ | cough \| NO<br>heart palpitations \| YES<br>tiredness or fatigue \| YES<br>dizziness \| NO<br>swelling in your legs ankles or feet \| NO<br>back pain \| NO<br>shortness of breath \| YES<br>spitting up of food from the esophagus or stomach<br>without nausea \| NO<br>restless legs syndrome \| NO<br>chest pressure \| YES<br>low blood pressure \| NO<br>fainting \| YES |
| Patient 400 | Heart disease | Cardiology | Female | 58 | hypertension | hypertension | | | | chest discomfort<br>chest pain | squeezing or aching sensation in your chest or<br>arms that may spread to your neck jaw or back \| YES<br>chest pressure \| NO<br>nausea or vomiting \| NO<br>shortness of breath \| YES<br>cough \| NO<br>pain radiates to jaw neck back or shoulders \| YES<br>arm pain or discomfort \| YES<br>rapid heartbeat \| YES<br>dizziness \| YES<br>anxiety \| NO<br>lightheadedness \| NO<br>throbbing headache \| NO<br>upper back pain \| NO<br>numbness in part of your body \| NO<br>chest pain worsened by exercise \| YES |
| Patient 401 | Hyperthyroidism | Diabetes / Endocrinology | Male | 45 | | | | | | sensitivity to heat<br>hyperactivity | anxiety \| NO<br>mood swings \| YES<br>rapid heartbeat \| YES<br>difficulty sleeping \| YES<br>dizziness \| YES<br>irritability \| YES<br>depression \| YES<br>weight loss \| YES<br>vomiting \| NO<br>sadness \| YES<br>fainting \| NO<br>shortness of breath or chest pain or palpitation<br>worsen when lying down \| YES<br>lethargy \| YES<br>pain in abdomen \| NO<br>extreme fatigue \| YES |
| Patient 402 | Hyperthyroidism | Diabetes / Endocrinology | Female | 46 | | ,,,,Hyperthyroid | | | | sensitivity to heat<br>mood swings<br>hyperactivity | anxiety \| YES<br>persistent tiredness and weakness \| YES<br>rapid heartbeat \| YES<br>sleep problems due to muscle cramps or restless legs \| YES<br>irritability \| YES<br>dizziness \| YES<br>weight loss \| NO<br>increased sensitivity to cold \| NO<br>weight gain \| NO<br>muscle aches and weakness \| NO<br>fainting \| NO<br>shortness of breath at rest \| NO<br>pain in abdomen \| NO<br>tiredness or fatigue \| YES<br>sharp pains or cramps in abdomen \| NO |
| Patient 403 | Liver disease | Hepatology | Male | 47 | | | | | | swelling of abdomen<br>nausea and vomiting<br>yellow skin and eyes | pain in upper abdomen \| YES<br>irritated skin around anus \| NO<br>cloudy or bloody urine \| NO<br>heartburn \| NO<br>urine retention \| NO<br>swelling in the belly legs and ankles \| YES<br>excess night urination \| NO<br>shortness of breath \| NO<br>unexplained fatigue \| YES<br>itchy skin \| YES |

# Supplementary Table 4

| | | | | | | | | | | | |
|---|---|---|---|---|---|---|---|---|---|---|---|
| Patient 404 | Liver disease | Hepatology | Female | 59 | | Liver disease | | | | pain in upper abdomen<br>dark stool<br>yellow skin and eyes | swelling of abdomen \| YES<br>nausea or vomiting \| YES<br>heartburn \| NO<br>belching \| YES<br>swelling in the belly legs and ankles \| YES<br>cloudy or bloody urine \| NO<br>excess night urination \| NO<br>shortness of breath \| NO<br>tiredness or fatigue \| YES<br>itchy skin \| YES<br>tiny red lines on the skin above waist \| YES<br>vomiting blood \| NO<br>weakness \| YES |
| Patient 405 | Stye | EYE / Ophthalmology | Male | 55 | | | | | | eyelid pain<br>red lump on eyelid | swollen eyelids \| YES<br>tearfulness \| YES |
| Patient 406 | Stye | EYE / Ophthalmology | Female | 56 | | | | | | tearfulness<br>swollen eyelids | red lump on eyelid \| YES<br>eyelid pain \| YES<br>red lump on eyelid \| YES |
| Patient 407 | Fibromyalgia | Rheumatology \|<br>Medicine / General Physician | Male | 36 | | | | | | pain all over the body<br>stiffness all over the body<br>difficulty sleeping | shortness of breath \| NO<br>neck pain \| YES<br>back pain \| YES<br>confusion \| YES<br>joint stiffness \| YES<br>sensitivity to light \| YES<br>sensitivity to sound \| YES<br>personality or behaviour changes \| NO<br>fainting \| NO<br>agitation \| NO<br>hip pain \| NO |
| Patient 408 | Fibromyalgia | Rheumatology \|<br>Medicine / General Physician | Female | 45 | | | | | | stiffness all over the body<br>difficulty concentrating<br>joint stiffness | pain in abdomen \| YES<br>increasing confusion \| YES<br>fainting \| NO<br>hip pain \| NO<br>lethargy \| NO<br>neck pain \| YES<br>back pain \| YES<br>unexplained fatigue \| YES<br>difficulty sleeping \| YES |
| Patient 409 | Hypothyroidism | Diabetes / Endocrinology | Male | 42 | | | | | | constipation or diarrhoea<br>increased sensitivity to cold<br>tiredness or fatigue | unexplained fatigue \| YES<br>sleepiness \| YES<br>dry skin \| YES<br>depression \| YES<br>sadness \| YES<br>weakness \| YES<br>anxiety \| NO<br>fainting \| NO<br>dizziness \| YES<br>vomiting \| NO<br>confusion \| YES<br>rapid heartbeat \| NO<br>lightheadedness \| YES<br>malaise \| YES |
| Patient 410 | Hypothyroidism | Diabetes / Endocrinology | Female | 44 | | Hypothyroidism | | | | increased sensitivity to cold<br>constipation<br>tiredness or fatigue | unexplained fatigue \| YES<br>dry skin \| YES<br>depression \| YES<br>sadness \| YES<br>nausea or vomiting \| YES<br>weakness \| YES<br>dizziness \| YES<br>anxiety \| YES<br>fainting \| NO<br>confusion \| NO<br>rapid heartbeat \| NO<br>lightheadedness \| NO<br>malaise \| NO<br>seizures \| NO<br>chills or shiver \| NO |
| Patient 411 | Laryngitis | ENT | Male | 38 | | | | | | hoarseness of voice<br>sore throat<br>dry throat | always needing to clear your throat \| YES<br>partial loss of voice \| YES<br>chronic cough \| YES<br>difficulty swallowing \| YES<br>difficulty speaking \| YES |
| Patient 412 | Laryngitis | ENT | Female | 38 | | | | | | hoarseness of voice<br>dry throat<br>sore throat | always needing to clear your throat \| YES<br>partial loss of voice \| YES<br>chronic cough \| YES<br>pain when swallowing \| YES<br>difficulty speaking \| YES |

# Supplementary Table 4

| | | | | | | | | | | | |
|---|---|---|---|---|---|---|---|---|---|---|---|
| Patient 413 | Hyperemesis gravic | Medicine / General Physician | Female | 28 | | | | | | feeling constant nausea<br>vomiting more than three times per day<br>dizziness | high blood pressure \| NO<br>poor appetite \| YES<br>pain in upper abdomen \| NO<br>low blood pressure \| YES<br>pregnant \| YES<br>weight loss \| YES<br>belching \| NO<br>severe headache \| NO<br>malaise \| YES<br>mild fever \| NO<br>pain in upper-right abdomen \| NO<br>constipation \| NO |
| Patient 414 | Hyperemesis gravic | Medicine / General Physician | Female | 30 | | | | | | dehydration<br>nausea and vomiting<br>pregnancy | weight loss \| YES<br>nausea and vomiting \| YES<br>weight loss \| YES |
| Patient 415 | Sciatica | Neuromedicine \|<br>Medicine / General Physician | Male | 33 | | | | | | pelvic pain<br>hip pain worsen with movement | numbness in part of your body \| YES<br>flank pain \| YES<br>hip pain \| YES<br>restricted movement \| YES<br>tenderness in the affected area \| NO<br>chronic back pain \| YES<br>weakness \| YES<br>pain increases with movement \| YES<br>pain increases at night \| NO<br>stiffness or pain in the neck \| NO<br>leg pain \| YES<br>loss of bladder or bowel control \| NO<br>urine leakage \| NO<br>discomfort \| YES<br>pain during urination \| NO |
| Patient 416 | Sciatica | Neuromedicine \|<br>Medicine / General Physician | Female | 45 | | | | | | pain in abdomen<br>pelvic pain<br>flank pain | numbness in part of your body \| YES<br>hip pain \| YES<br>restricted movement \| YES<br>tenderness in joint \| NO<br>chronic back pain \| YES<br>weakness \| YES<br>pain increases with movement \| YES<br>pain increases at night \| NO<br>stiffness or pain in the neck \| NO<br>leg pain \| YES<br>loss of bladder or bowel control \| NO<br>urine leakage \| NO<br>discomfort \| YES<br>pain during urination \| NO<br>falling \| NO |
| Patient 417 | Mastitis | Gynaecology \| Obstetric | Female | 28 | | | | | | hot and painful breast during touch<br>swelled area in breast | redness in breast \| YES<br>wedge shaped breast lump \| YES<br>burning pain in breast during breast feeding \| YES |
| Patient 418 | Mastitis | Gynaecology \| Obstetric | Female | 24 | | | | | | redness in breast<br>wedge shaped breast lump | swelled area in breast \| YES<br>hot and painful breast during touch \| YES<br>burning pain in breast during breast feeding \| YES |
| Patient 419 | Anemia | Haematology \|<br>Medicine / General Physician | Male | 33 | | | | | | recurrent episodes of mild to severe pain around joints<br>joint pain<br>unexplained fatigue | live or travelled recently to areas prone to viral fevers like<br>dengue malaria chikungunya or high prevalence of hepatitis (e.g. I<br>fluid in the abdomen \| NO<br>recurring episodes of pain in muscle or back or all over the body \|<br>headache \| NO<br>vomiting \| NO<br>pain in upper abdomen \| NO<br>pale skin \| YES<br>confusion \| NO<br>lethargy \| YES<br>back pain \| YES<br>recurrent infections \| YES<br>tiredness or fatigue \| YES<br>swelling of hands and feet \| YES<br>flapping tremor \| NO |

# Supplementary Table 4

| | | | | | | | | | | | |
|---|---|---|---|---|---|---|---|---|---|---|---|
| Patient 420 | Anemia | Haematology \|<br>Medicine / General Physician | Female | 45 | | | | | | yellow skin and eyes<br>anemia<br>live or travelled recently to areas prone to viral fevers<br>malaria<br>chikungunya or high prevalence of hepatitis (e.g. Indi | live or travelled recently to areas prone to viral fevers like<br>dengue malaria chikungunya or high prevalence<br>of hepatitis (e.g. India or Africa) \| NO<br>fluid in the abdomen \| NO<br>dark stool from digested blood \| YES<br>vomiting \| YES<br>pain in upper abdomen \| YES<br>swollen veins in the lower esophagus \| YES<br>confusion \| NO<br>lethargy \| YES<br>diarrhoea \| NO<br>discomfort in abdomen \| YES<br>vomiting blood \| YES<br>chills or shiver \| NO<br>tiredness or fatigue \| YES<br>bleeding \| NO<br>flapping tremor \| NO |
| Patient 421 | Liver disease | Hepatology | Male | 45 | | | | | | cloudy or bloody urine<br>easy bruising<br>yellow skin and eyes | live or travelled recently to areas prone to viral fevers<br>like dengue malaria chikungunya or high prevalence<br>of hepatitis (e.g. India or Africa) \| NO<br>high blood pressure \| YES<br>feeling of fullness in abdomen \| YES<br>increased size of your abdomen due to enlarged kidneys \| NO<br>morning headache \| NO |
| Patient 422 | Liver disease | Hepatology | Female | 36 | | | | | | pain in abdomen that may feel sharp or dull<br>unexplained fatigue<br>poor appetite | swelling in your legs ankles or feet \| YES<br>overweight \| YES<br>malaise \| YES<br>tenderness in abdomen \| YES<br>high blood pressure \| YES<br>feeling of fullness or burning in your abdomen \| NO<br>swelling in abdomen \| YES |
| Patient 423 | Conjunctivitis | EYE / Ophthalmology \|<br>Medicine / General Physician | Male | 55 | | | | | | eye pain<br>redness | high fever \| NO<br>throbbing headache \| NO<br>redness in one or both eyes \| YES<br>creamy white lesions on tongue \| NO<br>itching in one or both eyes \| YES<br>grittiness in one or both eyes \| YES<br>watery discharge from one or both eye \| YES<br>difficulty opening eyes in morning \| YES<br>tearfulness \| YES<br>swollen eyelids \| YES |
| Patient 424 | Conjunctivitis | EYE / Ophthalmology \|<br>Medicine / General Physician | Female | 33 | | | | | | swollen eyelids<br>eye pain<br>eyelid pain | eyelid pain \| NO<br>redness in one or both eyes \| YES<br>itching in one or both eyes \| YES<br>grittiness in one or both eyes \| YES<br>watery discharge from one or both eye \| YES<br>difficulty opening eyes in morning \| YES<br>tearfulness \| NO<br>burning in eye \| YES<br>sore throat \| NO<br>runny nose \| NO<br>trouble waking up \| YES<br>sensitivity to light \| YES<br>eye pain \| YES<br>fever \| YES |
| Patient 425 | Sciatica | Neuromedicine<br>Medicine / General Physician | Female | 44 | | | | | | difficulty walking<br>numbness or weakness in your lower back buttock leg | toe pain \| YES<br>swelling at big toe \| NO<br>swelling in the affected area \| NO<br>moderate to severe pain in lower back buttock and<br>down your leg \| YES<br>back pain \| YES<br>leg pain \| YES<br>restricted movement \| YES<br>pain increases with movement \| YES<br>numbness in leg \| YES<br>hip pain \| YES |
| Patient 426 | Sciatica | Neuromedicine<br>Medicine / General Physician | Male | 38 | | | | | | difficulty walking<br>numbness or weakness in your lower back buttock leg | moderate to severe pain in lower back buttock and<br>down your leg \| YES<br>hip pain \| YES<br>back pain \| YES<br>restricted movement \| YES<br>pain increases with movement \| YES<br>leg pain \| YES<br>numbness in leg \| YES |

# Supplementary Table 4

| | | | | | | | | | | | |
|---|---|---|---|---|---|---|---|---|---|---|---|
| Patient 427 | Psoriasis | Skin / Dermatology | Female | 36 | | | | | | dry skin<br>itchy skin<br>scaly plaques on the skin | cracked or scaly skin \| YES<br>bumps and blisters on skin \| NO<br>oozing on skin \| NO<br>crusting of the skin \| NO<br>thickened skin \| YES<br>bleeding from scratched skin \| YES |
| Patient 428 | Psoriasis | Skin / Dermatology | Male | 39 | | | | | | purple rashes on brown skin or pink or red rash on wh<br>dry skin<br>dry and cracked skin that may bleed | itchy skin \| YES<br>bumps and blisters on skin \| NO<br>oozing on skin \| NO<br>crusting of the skin \| NO<br>thickened skin \| NO<br>burning on skin \| NO |
| Patient 429 | Diabetes mellitus | Diabetes / Endocrinology | Female | 24 | | | | | | pregnancy<br>excess urination<br>excess thirst | weight loss \| NO<br>excess night urination \| YES<br>cuts or infection taking much longer to heal \| YES<br>fever \| NO<br>blurred vision \| YES<br>nausea or vomiting \| NO<br>recurrent infections \| YES<br>lethargy \| YES<br>diarrhoea \| YES<br>tiredness or fatigue \| YES<br>increased hunger \| YES<br>foot ulcer \| NO<br>odors from the affected area \| NO<br>dizziness \| YES<br>pain during urination \| NO |
| Patient 430 | Diabetes mellitus | Diabetes / Endocrinology | Female | 36 | | | | | | excess urination<br>excess night urination<br>pregnancy | pain during urination \| NO<br>weight loss \| NO<br>cuts or infection taking much longer to heal \| YES<br>tiredness or fatigue \| YES<br>thirst \| YES<br>increased hunger \| YES<br>blurred vision \| YES<br>foot ulcer \| NO<br>odors from the affected area \| NO<br>nausea and vomiting \| NO<br>fever \| NO<br>recurrent infections \| YES<br>lethargy \| YES<br>diarrhoea \| NO<br>dizziness \| YES |
| Patient 431 | Migraine | Neuromedicine | Female | 66 | | | | | | sensitivity to light<br>throbbing headache<br>nausea and vomiting | high blood pressure \| NO<br>lower back pain \| NO<br>severe headache \| YES<br>neck pain \| NO<br>lightheadedness \| NO<br>sudden paralysis numbness and weakness in<br>face arm or leg often one side of the body \| NO<br>dizziness \| NO<br>sensitivity to sound \| YES<br>fever \| NO<br>shortness of breath \| NO<br>pain in upper abdomen \| NO<br>bleeding from your nose without any injury \| NO |
| Patient 432 | Migraine | Neuromedicine | Female | 25 | | | | | | throbbing headache<br>headache and neck pain that lasts 3 days or longer<br>nausea and vomiting | shapes in vision \| YES<br>back pain \| NO<br>severe headache \| YES<br>flashes of light \| YES<br>lightheadedness \| NO<br>vomiting \| YES<br>dizziness \| NO<br>shortness of breath \| NO<br>chest pain \| NO<br>pain in upper abdomen \| NO<br>bleeding from your nose without any injury \| NO<br>sudden weight gain \| NO<br>sudden severe headache \| NO |

# Supplementary Table 4

| | | | | | | | | | | | |
|---|---|---|---|---|---|---|---|---|---|---|---|
| Patient 433 | Typhoid | Medicine / General Physician | Female | 22 | | | | | | persistent high fever<br>extreme fatigue<br>pain all over the body | live or travelled recently to areas prone to viral fevers like<br>dengue malaria chikungunya or high prevalence<br>of hepatitis (e.g. India or Africa) \| YES<br>dull pain in upper abdomen \| YES<br>muscle pain \| YES<br>cough with phlegm  \| NO<br>runny nose \| NO<br>yellow skin and eyes \| NO<br>sweating \| NO<br>sudden paralysis numbness and weakness in<br>face arm or leg often one side of the body \| NO<br>pain during urination \| NO<br>diarrhoea \| YES<br>bloating \| NO<br>severe headache \| NO<br>indigestion \| NO<br>constipation \| YES<br>high fever \| YES |
| Patient 434 | Typhoid | Medicine / General Physician | Male | 44 | | | | | | persistent high fever gradually increasing throughout t<br>nausea and vomiting<br>headache | pain all over the body \| YES<br>extreme fatigue \| YES<br>cough with phlegm \| NO<br>runny nose \| NO<br>dry cough \| YES<br>sore throat \| NO<br>live or travelled recently to areas prone to diseases<br>like meningitis (e.g. sub-Saharan Africa) \| YES<br>dull pain in upper-right abdomen \| NO<br>poor appetite \| YES<br>contact with typhoid patients \| NO<br>high fever \| YES<br>skin rash \| NO<br>sudden high fever \| NO<br>constipation \| YES<br>diarrhoea \| NO |
| Patient 435 | Diverticulosis | Gastroenterology | Female | 36 | | | | | | persistent pain in lower left side of the abdomen<br>pain in abdomen that gets worse after you eat<br>tenderness in abdomen | food intolerance \| YES<br>nausea and vomiting \| NO<br>fever \| YES<br>live or travelled recently to areas prone to diseases<br>like meningitis (e.g. sub-Saharan Africa) \| NO<br>constipation \| YES<br>blood in stool \| YES<br>feeling of fullness in abdomen \| NO<br>pain in upper abdomen \| NO<br>chest pain \| NO<br>vomiting blood \| NO |
| Patient 437 | Prolapse | Gynaecology | Female | 55 | | | | | | unable to completely empty your bladder<br>feeling that something is coming out of your vagina<br>pain during or after sex | pelvic pain \| YES<br>burning sensation during urination \| NO<br>sensation of heaviness or pulling in pelvis \| YES<br>pelvic pain \| YES<br>constipation \| YES<br>pain during urination \| NO<br>cloudy or bloody urine \| NO<br>decreased urine output \| NO<br>chills or shiver \| NO<br>nausea or vomiting \| NO |
| Patient 438 | Prolapse | Gynaecology | Female | 49 | | | | | | feeling that something is coming out of your vagina<br>sensation of heaviness or pulling in pelvis | pain during or after sex \| YES<br>urine retention \| NO<br>urine leakage \| NO<br>pelvic pain \| YES<br>constipation \| YES<br>feel like sitting on a small ball \| YES<br>lower abdomen discomfort \| YES<br>symptoms worsen as the day goes on \| YES<br>discomfort walking \| YES |
| Patient 439 | Epididymitis | Gynaecology | Male | 48 | | | | | | testicle pain<br>tenderness in scrotum | swelling in scrotum \| YES<br>pain during urination \| YES<br>groin pain \| YES<br>excess urination \| NO<br>recurrent infections \| NO<br>pain in lower abdomen \| YES<br>fever \| YES<br>chills or shiver \| NO<br>cloudy or bloody urine \| NO<br>nausea or vomiting \| NO<br>redness in the affected area \| YES<br>discomfort \| YES<br>lump \| NO<br>cyst \| NO<br>severe pain \| YES |

# Supplementary Table 4

| | | | | | | | | | | | |
|---|---|---|---|---|---|---|---|---|---|---|---|
| Patient 440 | Epididymitis | Gynaecology | Male | 55 | | | | N\A | | testicle pain<br>swelling in scrotum<br>tenderness in scrotum | pain during urination \| NO<br>groin pain \| YES<br>excess urination \| NO<br>recurrent infections \| NO<br>pain in lower abdomen \| YES<br>fever \| YES<br>chills or shiver \| NO<br>cloudy or bloody urine \| NO<br>nausea and vomiting \| YES<br>redness in the affected area \| YES<br>discomfort \| YES<br>lump \| NO<br>cyst \| NO<br>severe pain \| YES<br>flank pain \| YES |
| Patient 441 | Cardiac arrest | Cardiology | Female | 45 | heart_disease | | | | | rapid heartbeat<br>severe chest pain<br>irregular heartbeat | jaw pain \| YES<br>high blood pressure \| YES<br>cold sweat \| YES<br>squeezing or aching sensation in your chest or arms that may spread to your neck jaw or back \| YES<br>slow heart rate \| NO<br>chest pressure \| YES<br>nausea and vomiting \| YES<br>shortness of breath or chest pain or palpitation worsen when lying down \| YES<br>dizziness \| YES<br>anxiety \| NO<br>shoulder pain \| NO<br>chest discomfort \| YES<br>numbness in part of your body \| YES<br>arm pain or discomfort \| YES<br>depression \| YES |
| Patient 442 | Cardiac arrest | Cardiology | Male | 65 | heart_disease | | | | | chest pressure<br>chest pain<br>irregular heartbeat | severe squeezing or crushing chest pain \| YES<br>nausea and vomiting \| YES<br>shortness of breath \| YES<br>cough \| NO<br>pain radiates to jaw neck back or shoulders \| YES<br>chest pain worsened by exercise \| YES<br>arm pain or discomfort \| YES<br>chest discomfort \| YES<br>rapid heartbeat \| YES<br>dizziness \| YES<br>anxiety \| NO<br>lightheadedness \| NO<br>throbbing headache \| NO<br>upper back pain \| NO<br>numbness in part of your body \| NO |
| Patient 443 | Heart disease | Cardiology | Female | 39 | | | | | | chest pain<br>shortness of breath<br>chest tightness | arm pain or discomfort \| YES<br>swollen ankles feet or hands \| NO<br>cough \| NO<br>spitting up of food from the esophagus or stomach without nausea \| NO<br>dizziness \| YES<br>heart palpitations \| YES<br>lightheadedness \| NO<br>dizziness \| YES<br>lethargy \| YES<br>weight gain \| NO<br>tiredness or fatigue \| YES<br>anxiety \| NO |
| Patient 444 | Heart disease | Cardiology | Male | 40 | | | | | | severe chest pain<br>nausea and vomiting<br>chest discomfort | jaw pain \| YES<br>high blood pressure \| YES<br>cold sweat \| YES<br>squeezing or aching sensation in your chest or arms that may spread to your neck jaw or back \| YES<br>slow heart rate \| NO<br>chest pressure \| YES<br>shortness of breath at rest \| YES<br>dizziness \| YES<br>anxiety \| NO<br>rapid heartbeat \| NO<br>shoulder pain \| NO<br>numbness in part of your body \| NO<br>arm pain or discomfort \| YES<br>depression \| YES<br>sadness \| YES |

# Supplementary Table 4

| | | | | | | | | | | | |
|---|---|---|---|---|---|---|---|---|---|---|---|
| Patient 445 | Aphthous ulcer | Medicine / General Physician | Female | 55 | | | | | | a painful<br> burning sensation in the mouth<br>painful sores inside mouth or tongue or lips or your in | round ulcer white grey or yellow with red border \| YES |
| Patient 446 | Aphthous ulcer | Medicine / General Physician | Male | 45 | | | | | | painful sores inside mouth or tongue or lips or your in | round ulcer white grey or yellow with red border \| YES |
| Patient 447 | Endometriosis | Gynaecology | Female | 35 | | | | | | pelvic pain and cramping that start before period<br>pain during or after sex<br>nausea or vomiting | painful period \| YES<br>urine leakage \| NO<br>abnormal vaginal discharge \| NO<br>itching and irritation or fissure around the vagina \| NO<br>painful period \| YES<br>blood in urine during period \| YES<br>diarrhoea \| NO<br>constipation \| NO<br>cramping in abdomen \| YES<br>chills or shiver \| YES<br>pain during urination \| YES |
| Patient 448 | Endometriosis | Gynaecology | Female | 29 | | | | | | abnormal vaginal bleeding<br>pain during intercourse | bleeding after intercourse \| YES<br>abnormal vaginal discharge \| YES<br>bleeding between menstrual periods \| YES<br>pain during urination \| NO<br>fever \| NO<br>pain in abdomen \| YES<br>weakness \| YES<br>headache \| NO<br>nausea or vomiting \| NO<br>sadness \| YES<br>malaise \| YES |
| Patient 449 | Ovarian cyst | Gynaecology | Female | 38 | | | | | | severe and sharp pelvic pain<br>pelvic pain during bowel movement<br>sharp pains or cramps in abdomen | pain during urination \| YES<br>irregular heavy or lighter periods than normal \| YES<br>increased or decreased urination \| NO<br>cloudy or bloody urine \| NO<br>increased blood pressure \| NO<br>bloating \| YES<br>chronic pelvic pain \| YES<br>swollen belly \| YES<br>nausea and vomiting \| YES<br>pain during sex \| YES<br>tiredness or fatigue \| YES |
| Patient 450 | Ovarian cyst | Gynaecology | Female | 24 | | | | | | pain during or after sex<br>pain during urination<br>pelvic pain | urine retention \| NO<br>urine leakage \| NO<br>feeling that something is coming out of your vagina \| NO<br>sensation of heaviness or pulling in pelvis \| YES<br>severe and sharp pelvic pain \| YES<br>pelvic pain during bowel movement \| YES<br>lower abdomen discomfort \| YES<br>frequent need to urinate \| NO<br>excess urination \| NO |
| Patient 451 | Dementia | Neuromedicine | Female | 24 | | | | | | memory loss of recent events<br>increasing confusion | loss of ability to do everyday tasks \| YES<br>problems with recognition \| YES<br>poor concentration \| YES<br>problems with spatial awareness \| YES<br>depression \| YES<br>cognitive deficits \| NO<br>apathy and withdrawal \| NO<br>personality or behaviour changes \| NO<br>fainting \| NO<br>agitation \| NO<br>hip pain \| NO<br>lethargy \| NO<br>delirium \| NO<br>low blood pressure \| NO<br>easy bruising \| NO |

# Supplementary Table 4

| | | | | | | | | | | | |
|---|---|---|---|---|---|---|---|---|---|---|---|
| Patient 452 | Dementia | Neuromedicine | Male | 55 | | | | | | memory loss of recent events<br>problems with recognition<br>problems with spatial awareness | confusion \| YES<br>increasing confusion \| YES<br>loss of ability to do everyday tasks \| YES<br>poor concentration \| YES<br>depression \| YES<br>cognitive deficits \| NO<br>apathy and withdrawal \| NO<br>personality or behaviour changes \| NO<br>fainting \| NO<br>agitation \| NO<br>hip pain \| NO<br>lethargy \| NO<br>delirium \| NO<br>low blood pressure \| NO<br>easy bruising \| NO |
| Patient 453 | Spondylosis | Neuromedicine \| Orthopedic | Female | 36 | | | | | | weakness numbness arms hands or fingers<br>neck pain<br>neck pain that may travel to your arms or shoulders | grinding or popping feeling when moving the spine \| YES<br>difficulty walking \| YES<br>weakness in the hands or legs \| YES<br>back pain \| NO<br>loss of bladder or bowel control \| NO<br>numbness in part of your body \| YES<br>problems with coordination \| YES<br>muscle pain \| YES<br>throbbing headache \| NO<br>depression \| NO<br>sadness \| NO<br>dizziness \| NO<br>loss of bladder or bowel control \| NO<br>fainting \| NO<br>shoulder pain \| YES |
| Patient 454 | Spondylosis | Neuromedicine \| Orthopedic | Male | 45 | | | | | | weakness in the hands or legs<br>neck pain<br>grinding or popping feeling when moving the spine | neck pain that may travel to your arms or shoulders \| YES<br>difficulty walking \| YES<br>back pain \| YES<br>loss of bladder control \| NO<br>numbness in part of your body \| YES<br>problems with coordination \| YES<br>muscle pain \| NO<br>throbbing headache \| NO<br>depression \| NO<br>sadness \| NO<br>dizziness \| NO<br>loss of bladder or bowel control \| NO<br>fainting \| YES<br>shoulder pain \| YES<br>arm pain or discomfort \| YES |
| Patient 455 | Kidney disease | Nephrology | Female | 55 | | | | | | cloudy or bloody urine<br>high blood pressure<br>back pain | feeling of fullness or burning in your abdomen \| NO<br>swelling in leg or ankle \| NO<br>increased size of your abdomen due to enlarged kidneys \| YES<br>morning headache \| NO |
| Patient 456 | Kidney disease | Nephrology | Male | 48 | | | | | | cloudy or bloody urine<br>increased size of your abdomen due to enlarged kidney<br>back pain | high blood pressure \| YES<br>feeling of fullness or burning in your abdomen \| NO<br>morning headache \| NO |
| Patient 463 | Diarrhoea | Medicine / General Physician | Female | 66 | | | | N\A | | sunken eyes<br>dehydration<br>frequently pass watery or loose stool | sharp pains or cramps in abdomen \| YES<br>nausea and vomiting \| NO<br>poor appetite \| YES<br>muscle cramps \| YES<br>drowsiness \| YES<br>headache \| NO<br>tiredness or fatigue \| YES<br>dizziness \| YES<br>pale or mottled skin \| NO<br>irritability \| YES |
| Patient 464 | Diarrhoea | Medicine / General Physician | Male | 25 | | | | | | dehydration<br>frequently pass watery or loose stool<br>muscle cramps | sharp pains or cramps in abdomen \| YES<br>nausea and vomiting \| NO<br>poor appetite \| YES<br>sunken eyes \| YES<br>muscle cramps \| YES<br>headache \| NO<br>tiredness or fatigue \| YES<br>dizziness \| YES<br>pale or mottled skin \| NO<br>rapid heartbeat \| YES<br>irritability \| YES |

Supplementary Table 4

| | | | | | | | | | | | |
|---|---|---|---|---|---|---|---|---|---|---|---|
| Patient 465 | Gastritis | Gastroenterology | Female | 45 | | | | | | dark stool from digested blood<br>vomiting | swelling in leg or ankle \| NO<br>yellow skin and eyes \| NO<br>pain in abdomen \| YES<br>belching \| YES<br>feeling of fullness or burning in your abdomen \| YES<br>pain in upper abdomen \| YES<br>poor appetite \| YES<br>diarrhoea \| NO<br>chills or shiver \| NO<br>vomiting blood \| YES<br>tenderness in the affected area \| NO<br>discomfort \| YES<br>constipation \| YES<br>cramping \| YES<br>anxiety \| NO |
| Patient 466 | Gastritis | Gastroenterology | Male | 25 | | | | | | pain in abdomen<br>vomiting blood<br>nausea and vomiting | joint pain \| NO<br>belching \| YES<br>feeling of fullness or burning in your abdomen \| YES<br>pain in upper abdomen \| YES<br>indigestion \| YES<br>diarrhoea \| NO<br>chills or shiver \| YES<br>discomfort in upper abdomen \| YES<br>tenderness in the affected area \| NO<br>constipation \| NO<br>cramping \| YES<br>anxiety \| YES<br>depression \| YES<br>sadness \| YES<br>dizziness \| NO |
| Patient 467 | Acne vulgaris | Skin / Dermatology | Female | 45 | | | | | | pimples with pus at their tips<br>crusting | whitehead on your face \| YES<br>blackheads on your face and forehead \| YES<br>lump \| NO<br>small painless bumps beneath the skin \| YES<br>problems with self esteem \| YES<br>dark spots on your face \| YES<br>anxiety \| YES<br>depression \| YES |
| Patient 468 | Acne vulgaris | Skin / Dermatology | Male | 55 | | | | | | blackheads on your face and forehead<br>pimples with pus at their tips<br>crusting | whitehead on your face \| YES<br>large solid painful lumps under the skin \| YES<br>small red tender bumps under skin on your face \| YES<br>problems with self esteem \| YES<br>dark spots on your face \| YES |
| Patient 469 | Epilepsy | Neuromedicine | Female | 38 | | | | | | loss of consciousness or awareness<br>uncontrollable jerking movements of the arms and legs<br>stiffness | seizures \| YES<br>staring spells \| NO<br>fear \| NO<br>fainting \| YES<br>anxiety \| NO<br>falling \| YES<br>throbbing headache \| NO<br>depression \| YES<br>sadness \| YES<br>brief visual or sensory abnormality \| YES<br>confusion \| YES<br>weakness \| YES<br>loss of bladder or bowel control \| NO<br>tiredness or fatigue \| NO<br>agitation \| NO |
| Patient 470 | Epilepsy | Neuromedicine | Male | 39 | | | | | | stiffness<br>fainting<br>total or limited loss of consciousness | uncontrollable jerking movements of the arms and legs \| YES<br>staring spells \| NO<br>fear \| NO<br>anxiety \| NO<br>falling \| YES<br>throbbing headache \| NO<br>depression \| NO<br>sadness \| NO<br>brief visual or sensory abnormality \| YES<br>confusion \| YES<br>weakness \| YES<br>loss of bladder or bowel control \| NO<br>tiredness or fatigue \| NO<br>dizziness \| NO<br>agitation \| NO |

# Supplementary Table 4

| | | | | | | | | | | | |
|---|---|---|---|---|---|---|---|---|---|---|---|
| Patient 471 | Diphtheria | ENT | Female | 15 | | | | | | difficulty speaking<br>swollen glands<br>a thick grey-white coating that is covering the back of nose and tongue | high fever \| YES<br>swelling in the neck \| YES<br>live or travelled recently to areas prone to diseases like meningitis (e.g. sub-Saharan Africa) \| NO<br>difficulty swallowing \| YES<br>sore throat \| YES<br>difficulty breathing \| YES<br>pus filled blisters on your legs feet and hands \| NO<br>large ulcers surrounded by red sore looking skin \| NO<br>malaise \| YES<br>nasal discharge \| NO |
| Patient 472 | Diphtheria | ENT | Male | 25 | | | | | | a thick grey-white coating that is covering the back of nose and tongue<br>high fever<br>swelling in the neck | swollen throat \| YES<br>bad breath \| NO<br>red swollen tonsils \| NO<br>cough \| NO<br>nasal discharge \| NO<br>sore throat \| YES<br>muffled or throaty voice \| NO<br>throat pain \| YES<br>large ulcers surrounded by red sore looking skin \| YES<br>ear pain \| NO<br>headache \| NO<br>drooling \| NO<br>poor appetite \| YES<br>pain in abdomen \| NO<br>live or travelled recently to areas prone to viral fevers like dengue malaria chikungunya or high prevalence of hepatitis (e.g. India or Africa) \| YES |
| Patient 473 | Headache | Medicine / General Physician | Female | 65 | | | | | | headache<br>tenderness in the affected area | bleeding from your nose without any injury \| NO<br>sudden severe headache \| YES<br>high fever \| NO<br>live or travelled recently to areas prone to diseases like meningitis (e.g. sub-Saharan Africa) \| NO<br>pale or mottled skin \| NO<br>cold hands and feet \| NO<br>skin rash \| NO<br>high blood pressure \| NO<br>yellow skin and eyes \| NO<br>pain in lower abdomen \| NO<br>stiffness or pain in the neck \| NO<br>speak in short or incomplete sentence \| NO<br>blurred vision \| NO<br>malaise \| YES |
| Patient 475 | Adenomyosis | Gynaecology | Female | 35 | | | | | | heavy bleeding during menstrual period<br>pain during menstrual period<br>pain during sex | pelvic pain \| YES<br>nausea or vomiting \| YES<br>severe pain in abdomen \| YES<br>chills or shiver \| YES<br>pain during urination \| NO<br>blood in urine during period \| NO<br>blood in urine \| NO |
| Patient 476 | Adenomyosis | Gynaecology | Female | 39 | | | | | | pain during or after sex<br>chronic pelvic pain | urine retention \| NO<br>urine leakage \| NO<br>abnormal vaginal discharge \| NO<br>menstrual cramps \| YES<br>pain during menstrual period \| YES<br>constipation \| NO<br>nausea or vomiting \| YES<br>lower abdomen discomfort \| YES<br>fever \| YES<br>discomfort walking \| YES<br>chills or shiver \| YES |
| Patient 477 | Lung Disease | Respiratory / Chest Disease | Female | 45 | | | | | | heart palpitations<br>shortness of breath at rest<br>dizziness | jaw pain \| NO<br>chest pain \| YES<br>swelling in your legs ankles or feet \| YES<br>nausea and vomiting \| NO<br>blurred vision \| YES<br>cough \| NO<br>severe headache \| YES<br>wheezing \| YES<br>chest discomfort \| YES<br>rapid heartbeat \| YES<br>anxiety \| YES<br>arm pain or discomfort \| NO |

# Supplementary Table 4

| | | | | | | | | | | | |
|---|---|---|---|---|---|---|---|---|---|---|---|
| Patient 478 | Lung Disease | Respiratory / Chest Disease | Male | 46 | | | | | | blue or gray skin color due to low oxygen levels<br>chest pain<br>neck pain | dizziness \| YES<br>nausea and vomiting \| NO<br>shortness of breath at rest \| YES<br>cough \| YES<br>chest pain worsened by exercise \| YES<br>tiredness or fatigue \| YES<br>chest discomfort \| YES<br>rapid heartbeat \| YES<br>dizziness \| NO<br>anxiety \| NO<br>lightheadedness \| YES<br>throbbing headache \| NO<br>heart palpitations \| YES<br>arm pain or discomfort \| YES<br>cough with phlegm \| NO |
| Patient 479 | Epistaxis | ENT | Female | 48 | | | | | | bleeding from your nose without any injury<br>headache<br>blowing your nose with force | sinus pain \| YES<br>picked your nose \| YES<br>yellow skin and eyes \| NO<br>being at high high altitudes \| NO<br>cough \| NO<br>headache \| YES<br>changes in humidity or temperature causing the inside of the nose to become dry and cracked \| YES<br>arm pain or discomfort \| YES<br>cough with phlegm \| NO |
| Patient 481 | Dementia | Neuromedicine | Female | 47 | | | | | | memory loss<br>wandering and getting lost | memory loss of recent events \| YES<br>confusion \| YES<br>increasing confusion \| YES<br>loss of ability to do everyday tasks \| YES<br>problems with recognition \| YES<br>poor concentration \| YES<br>problems with spatial awareness \| YES<br>depression \| YES<br>cognitive deficits \| YES<br>apathy and withdrawal \| NO<br>personality or behaviour changes \| NO<br>fainting \| NO<br>agitation \| NO<br>hip pain \| NO<br>lethargy \| NO |
| Patient 482 | Respiratory infectic | Respiratory / Chest Disease | Male | 35 | | | | | | cough with phlegm<br>runny nose<br>sore throat | mild fever \| YES<br>body ache \| YES<br>headache \| YES<br>sneezing \| YES<br>shortness of breath \| NO<br>wheezing \| NO<br>heart palpitations \| NO<br>arm pain or discomfort \| YES<br>cough with phlegm \| NO |
| Patient 483 | Respiratory infectic | Respiratory / Chest Disease | Female | 39 | | | | | | runny or stuffy nose<br>persistent cough<br>headache | bleeding from your nose without any injury \| NO<br>coughing up blood \| NO<br>mild fever \| YES<br>cough with phlegm \| NO<br>dry cough \| NO<br>sore throat \| NO<br>muscle pain \| NO<br>body ache \| NO<br>tiredness or fatigue \| NO<br>difficulty sleeping \| YES<br>poor appetite \| YES<br>diarrhoea \| YES<br>arm pain or discomfort \| YES<br>cough with phlegm \| NO |
| Patient 484 | Respiratory infectic | Respiratory / Chest Disease | Male | 24 | | | | | | cough with phlegm<br>runny nose<br>sore throat | nasal congestion \| YES<br>body ache \| YES<br>headache \| YES<br>mild fever \| YES<br>excess mucus \| YES<br>chills or shiver \| NO<br>wheezing \| NO<br>headache \| NO<br>chest pain \| NO<br>chest pressure \| YES<br>nausea and vomiting \| NO<br>arm pain or discomfort \| YES<br>cough with phlegm \| NO |
| Patient 485 | Pre-eclampsia | Gynaecology | Female | 25 | | | | | | high blood pressure<br>vision problems<br>pregnant | pain just below the ribs \| YES |

# Supplementary Table 4

| | | | | | | | | | | | |
|---|---|---|---|---|---|---|---|---|---|---|---|
| Patient 486 | Pre-eclampsia | Gynaecology | Female | 28 | | hypertension | | | | swelling in extremities<br>sudden weight gain<br>sudden swelling of face | headache \| YES<br>neck pain \| NO<br>lightheadedness \| YES<br>dizziness \| YES<br>chest pain \| NO<br>tiredness or fatigue \| YES<br>nose bleed \| NO<br>shortness of breath \| NO<br>cloudy or bloody urine \| NO<br>arm pain or discomfort \| NO<br>sensitivity to light \| YES<br>nausea and vomiting \| YES<br>pregnant \| YES<br>arm pain or discomfort \| YES<br>cough with phlegm \| NO |
| Patient 487 | Rhabdomyolysis | Medicine / General Physician | Female | 26 | | hypertension | | | | dark orange brown tea-colored urine<br>muscle swelling<br>muscle spasms and pain | high blood pressure \| NO<br>cramping \| YES<br>leg pain \| YES<br>numbness in part of your body \| YES<br>burning sensation or pain during urination \| NO<br>discomfort in your lower back or abdomen \| NO<br>small amount of urine \| NO<br>muscle weakness \| YES<br>fever \| NO<br>nausea and vomiting \| NO<br>unexplained fatigue \| YES<br>arm pain or discomfort \| YES<br>cough with phlegm \| NO |
| Patient 489 | Ear infection | ENT | Female | 28 | | | | | | fluid draining from ear<br>tugging in one or both ear<br>rritability | ear pain \| YES<br>fever \| YES<br>hearing difficulties \| YES<br>itching and irritation in and around the ear \| YES<br>scaly skin in and around the ear \| YES |
| Patient 490 | Ear infection | ENT | Male | 55 | | | | | | ear pain<br>fluid draining from ear<br>hearing difficulties | mild fever \| YES<br>itching and irritation in and around the ear \| YES<br>tugging in one or both ear \| YES<br>scaly skin in and around the ear \| YES |
| Patient 491 | Contact dermatitis | Skin / Dermatology | Female | 45 | | | | | | leathery patches on skin that are darker than usual<br>bumps and blisters on skin<br>an itchy rash on your skin | swelling on skin \| YES<br>inflammation on skin \| YES<br>redness on skin \| YES<br>thickened skin \| YES<br>burning sensation during urination \| YES<br>skin exposed to chemicals or substance \| YES<br>purple or grey color skin \| YES |
| Patient 492 | Contact dermatitis | Skin / Dermatology | Male | 36 | | | | | | bumps and blisters on skin<br>itchy skin | swelling on skin \| YES<br>inflammation on skin \| YES<br>redness on skin \| YES<br>thickened skin \| YES<br>burning sensation during urination \| YES<br>skin exposed to chemicals or substance \| YES<br>purple or grey color skin \| YES<br>itchy skin \| YES |
| Patient 501 | Stroke | Neuromedicine \|<br>Medicine / General Physician | Male | 73 | hypertension | hypertension | Anti hypertensive | | | memory loss of recent events<br>loss of ability to do everyday tasks<br>problems with recognition | poor concentration \| YES<br>personality or behaviour changes \| YES<br>fainting\| NO<br>problems with recognition \| YES<br>wandering and getting lost \| YES<br>problems with spatial awareness \| YES<br>loss of bladder or bowel control \| NO<br>paranoid delusions \| NO<br>unexplained fatigue \| NO<br>headache \| NO<br>agitation \| YES<br>difficulty walking \| NO |
