# Supplementary material for: AmarDoctor: An AI-Driven, Multilingual, Voice-Interactive Digital Health Application for Primary Care Triage and Patient Management to Bridge the Digital Health Divide for Bengali Speakers
Source: arXiv:2510.24724 source file (2025-09-28)
Supplement: Supplementary file 3 [file Supplementary_Materials.tex]

\documentclass[12pt]{article}
\usepackage{pdfpages}    % for including external PDFs
\usepackage{appendix}    % for formatting appendix sections

\begin{document}

\appendix

\includepdf[pages=-]{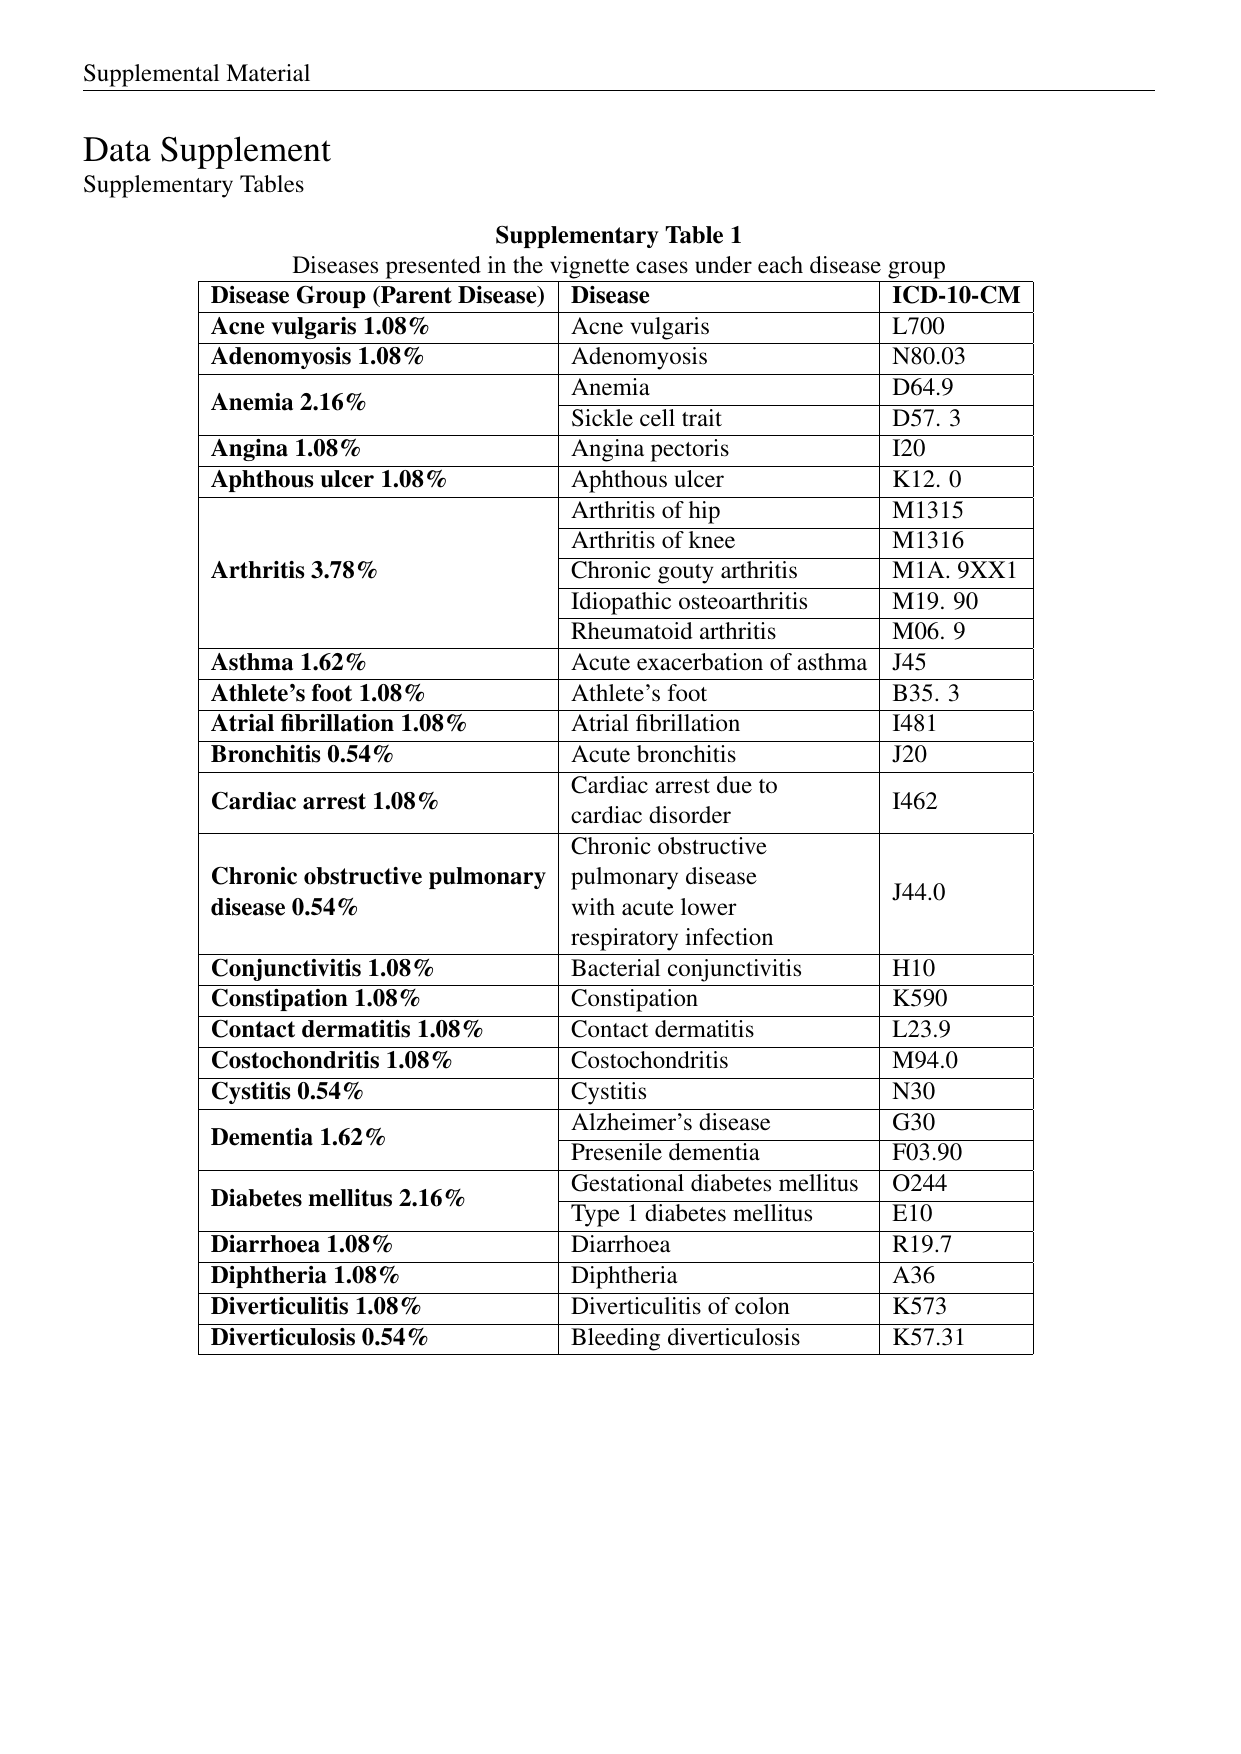}
\includepdf[pages=-]{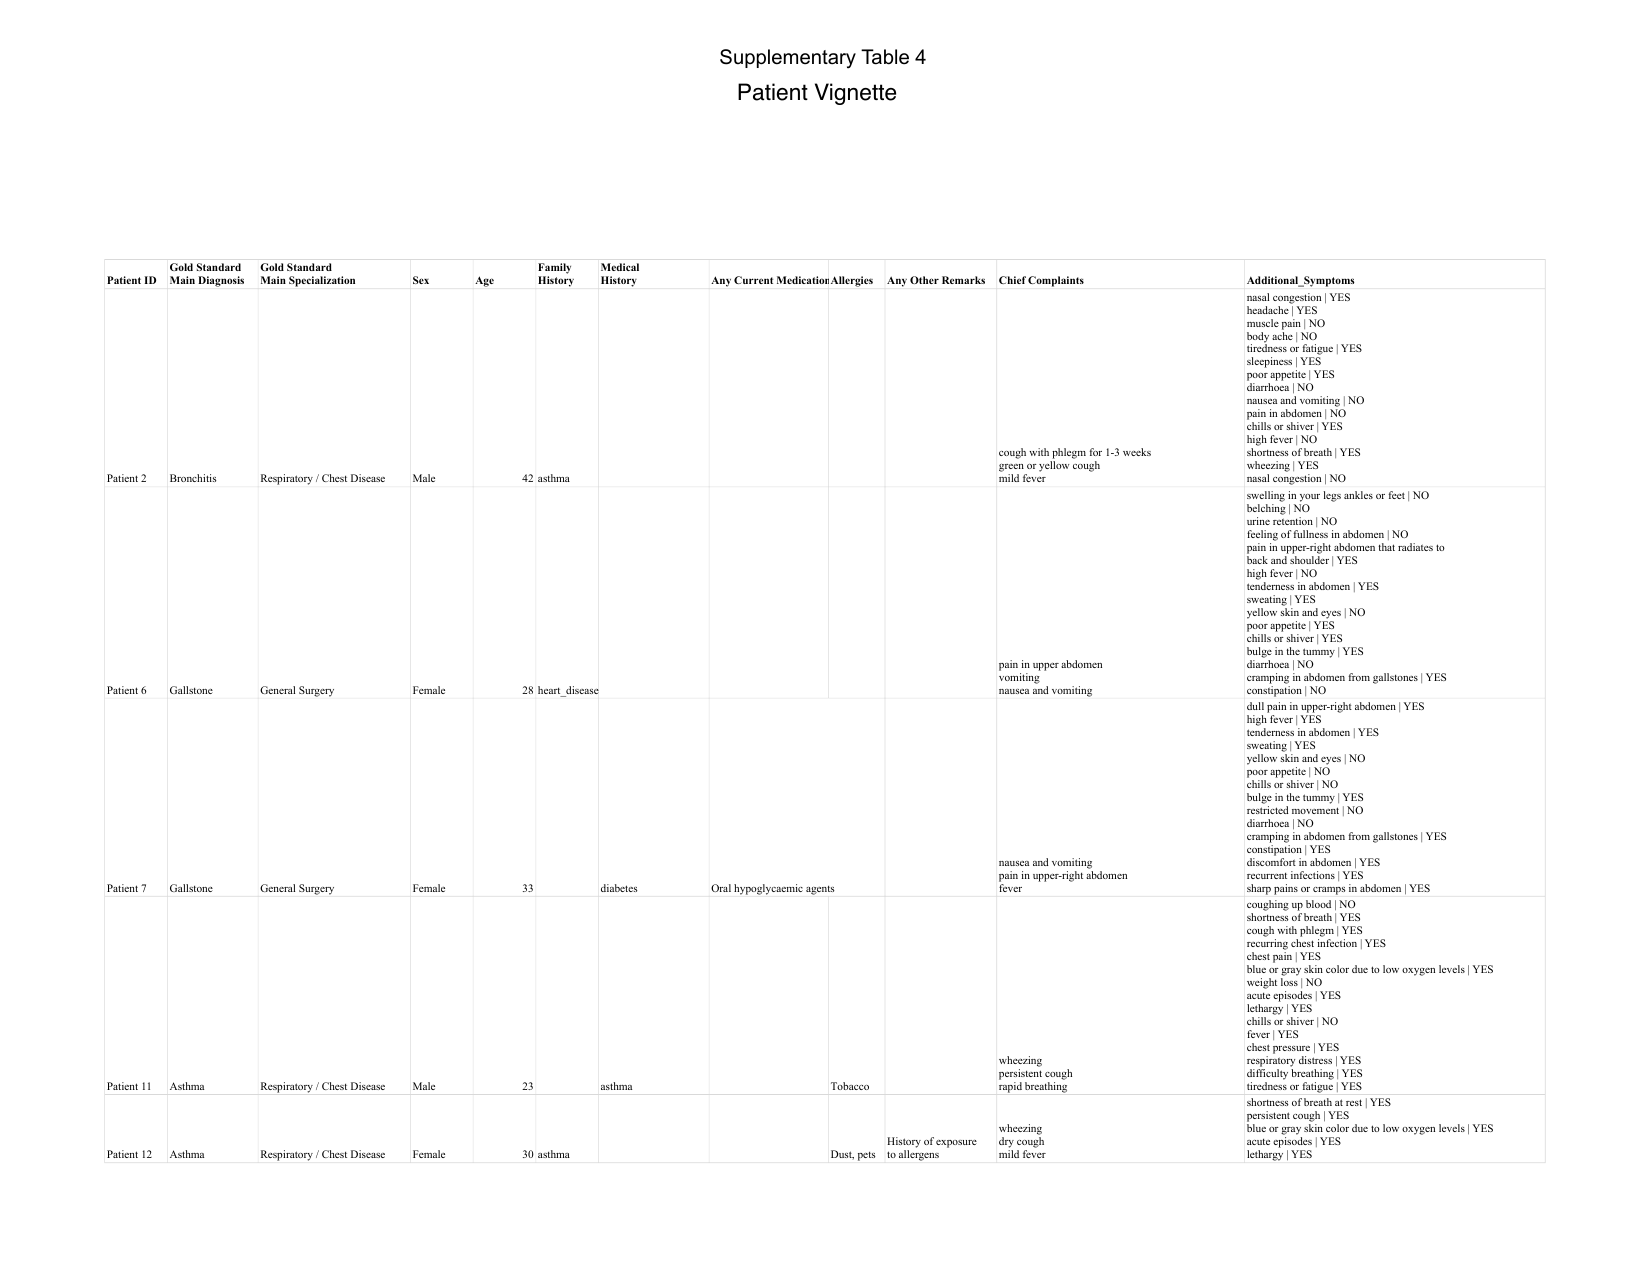}

\end{document}
